# Supplementary material for: Patch-based 3D Natural Scene Generation from a Single Example
Source: arXiv:2304.12670 source file (2023-04-26)
Supplement: Supplementary file 1 [file supplementary_alpha_effects.pdf]

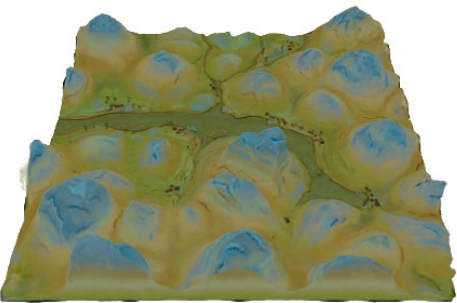

$\alpha = 0.005$

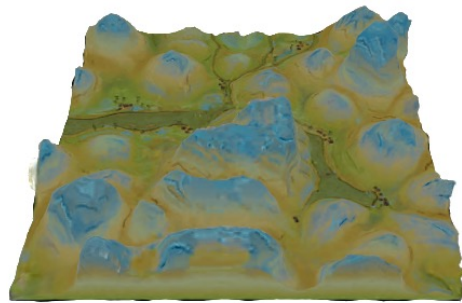

$\alpha = 0.05$

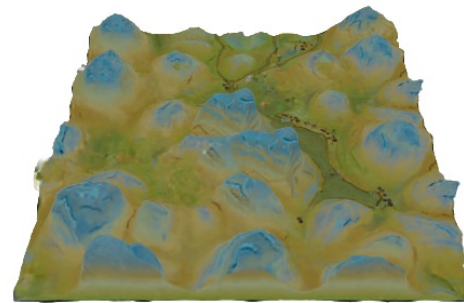

$\alpha = 0.5$

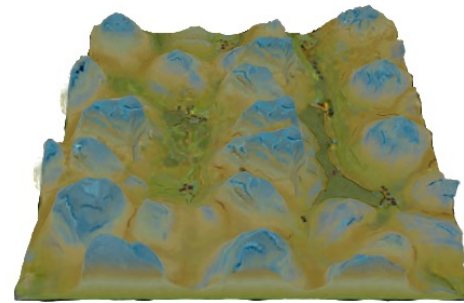

$\alpha = 1.0$

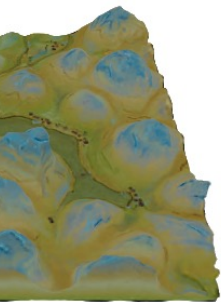

$\alpha = 0.005$

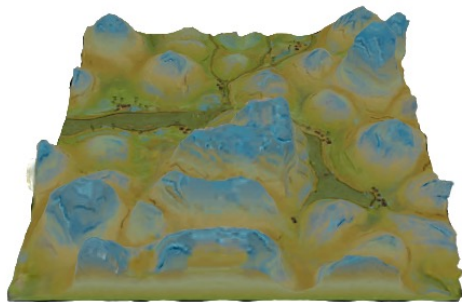

$\alpha = 0.05$

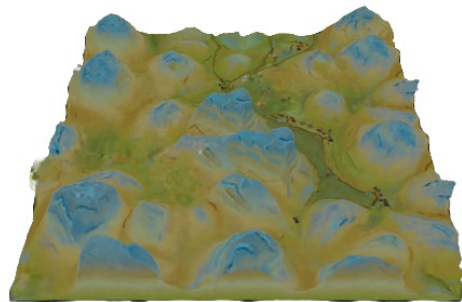

$\alpha = 0.5$

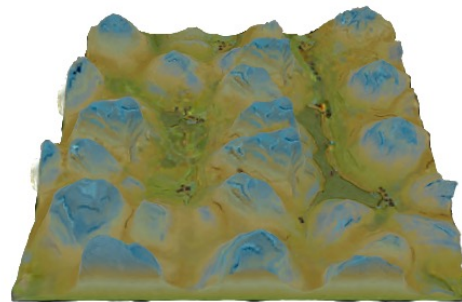

$\alpha = 1.0$

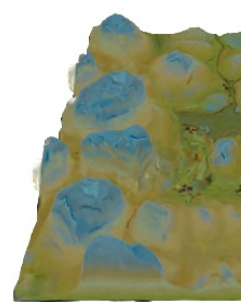

$\alpha = 2.0$
