# Supplementary material for: Patch-based 3D Natural Scene Generation from a Single Example
Source: arXiv:2304.12670 source file (2023-04-26)

Cactus Cereus

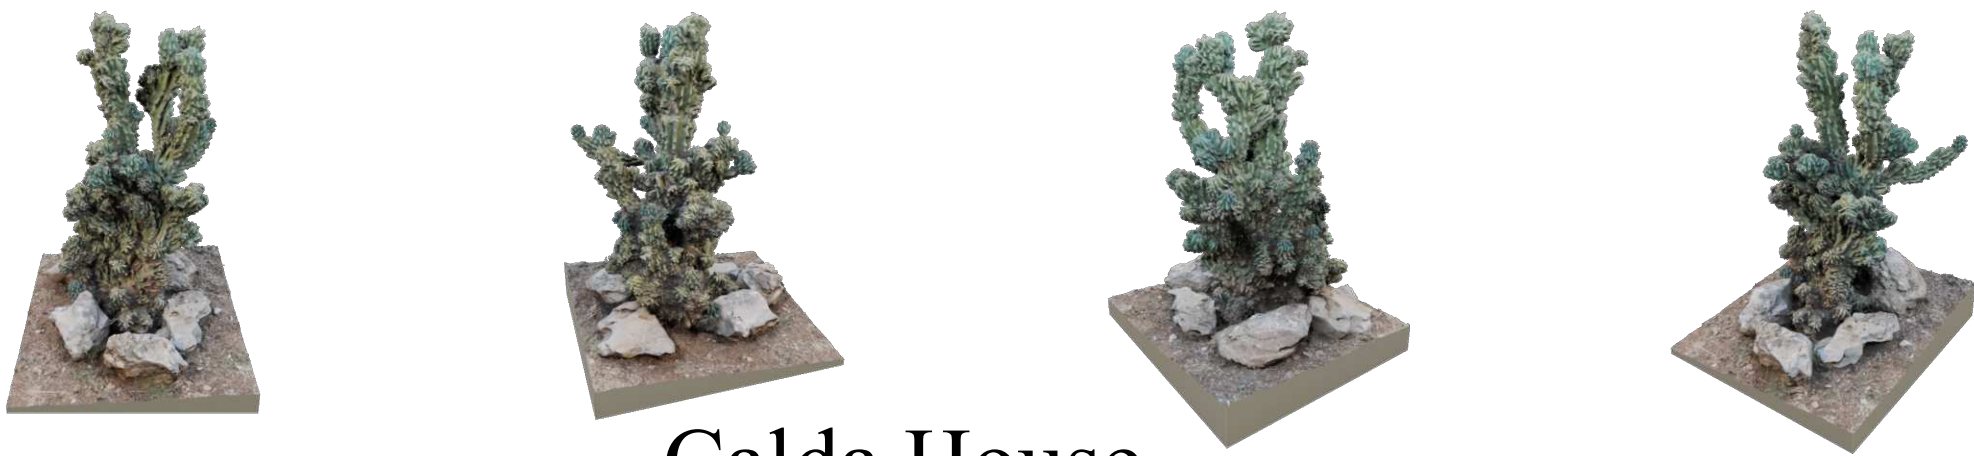

Cactus Saguaro

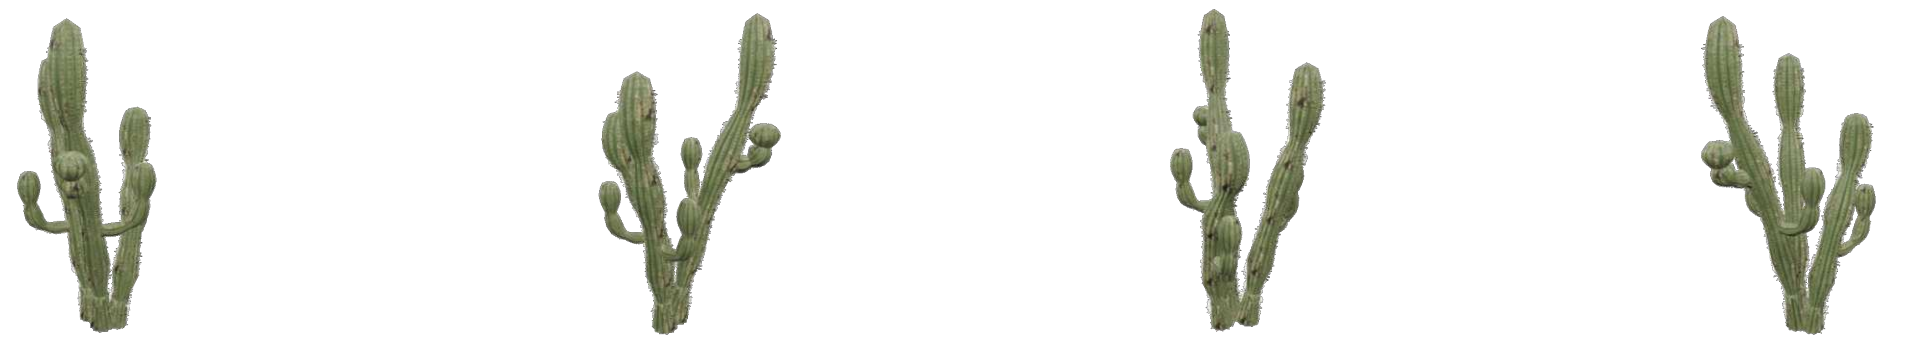

Calda House

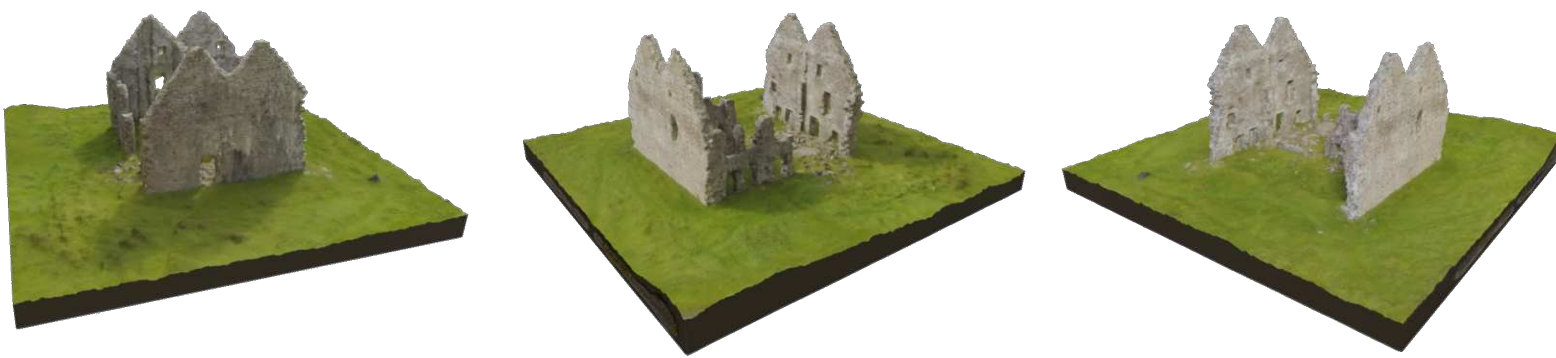

Callanish

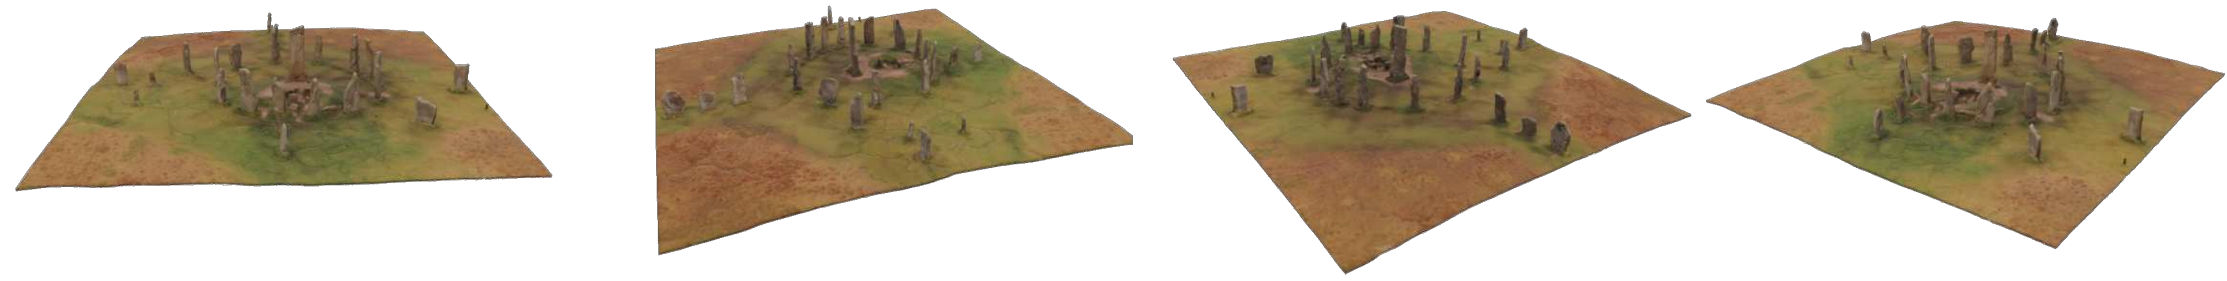

Camping Lowpoly

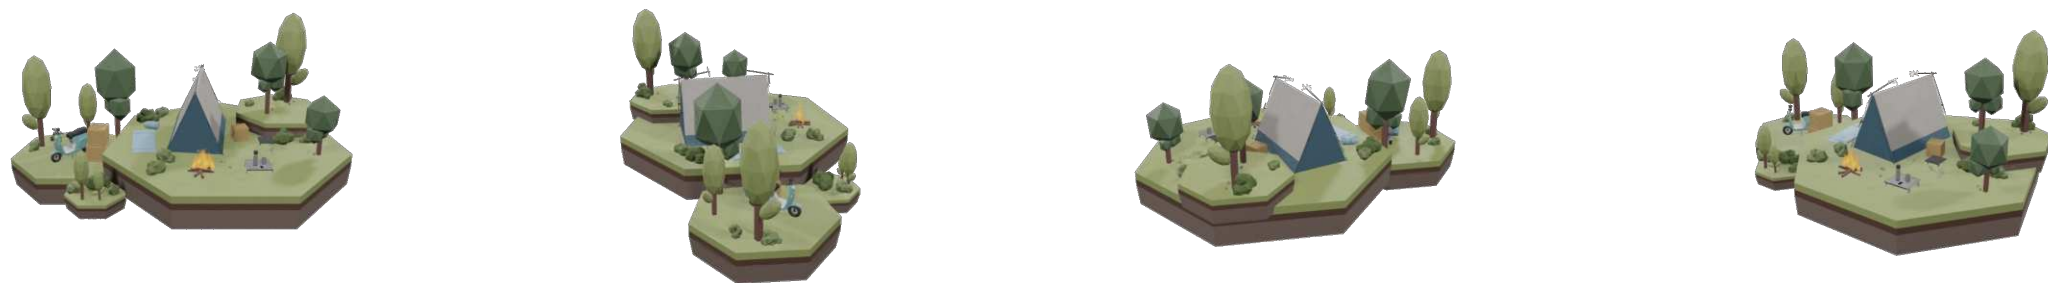

Desert Lowpoly

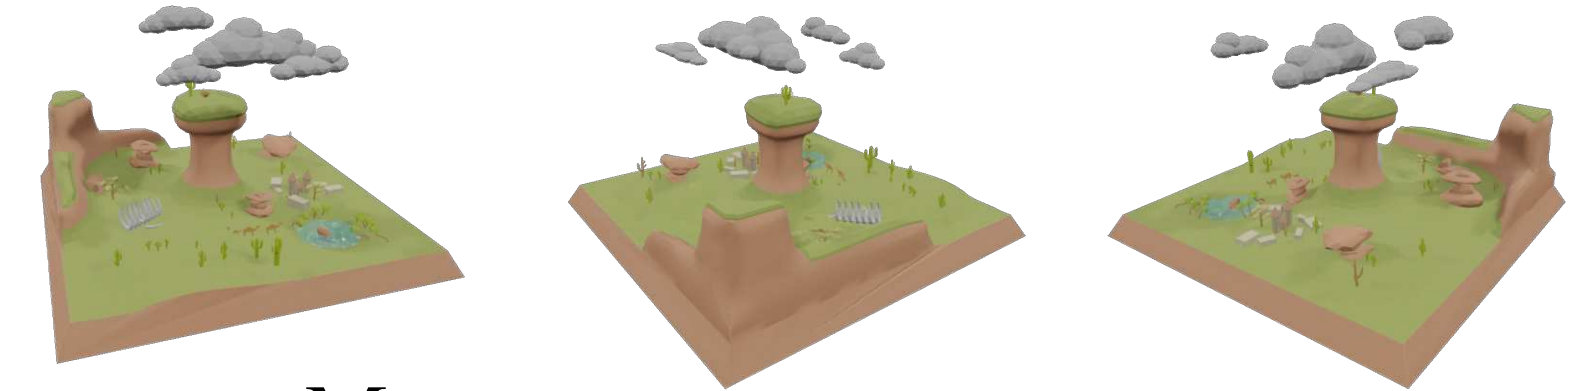

Green Island

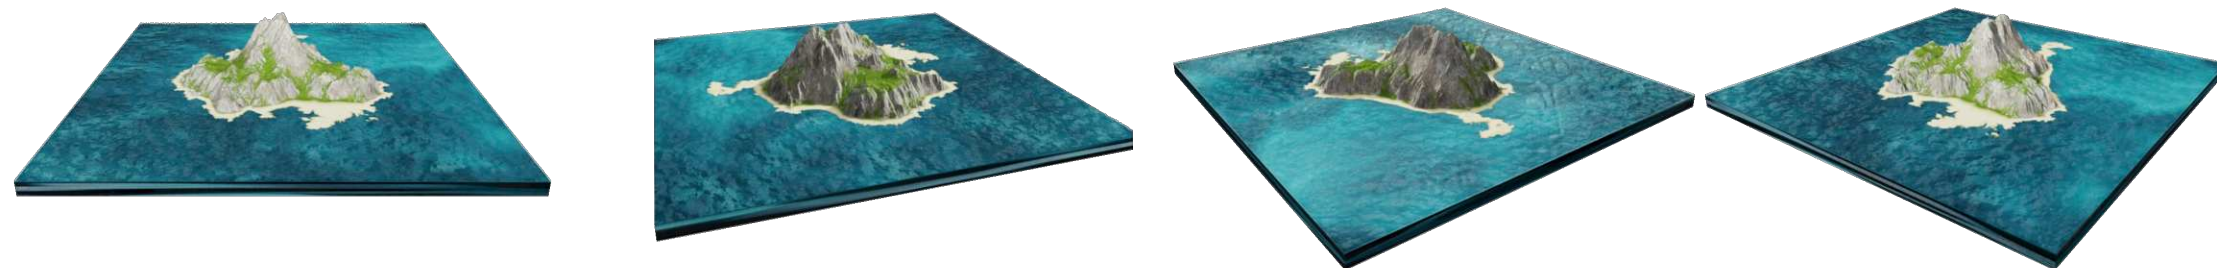

Meteora

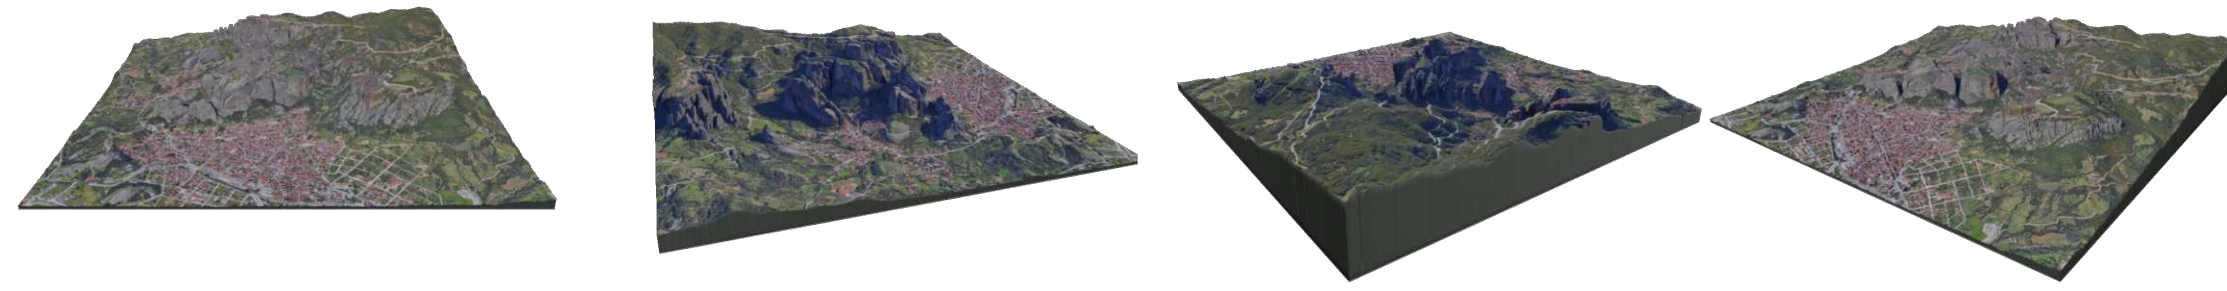

Mountain

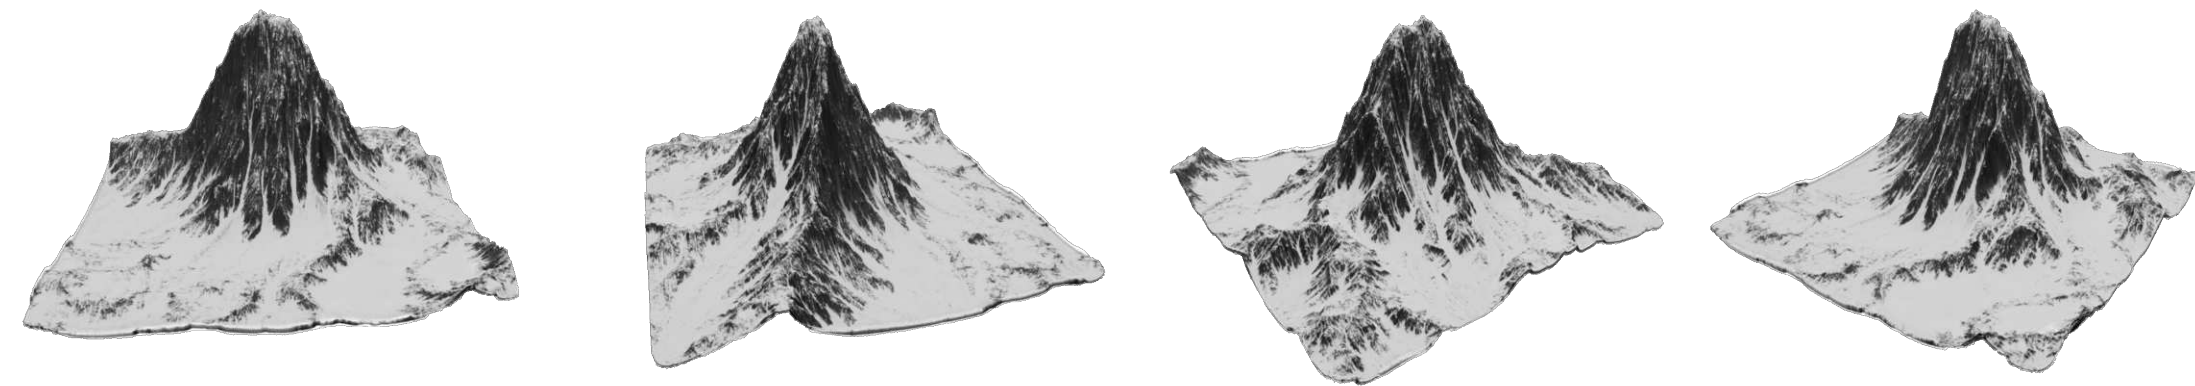

Mountain with Lakes

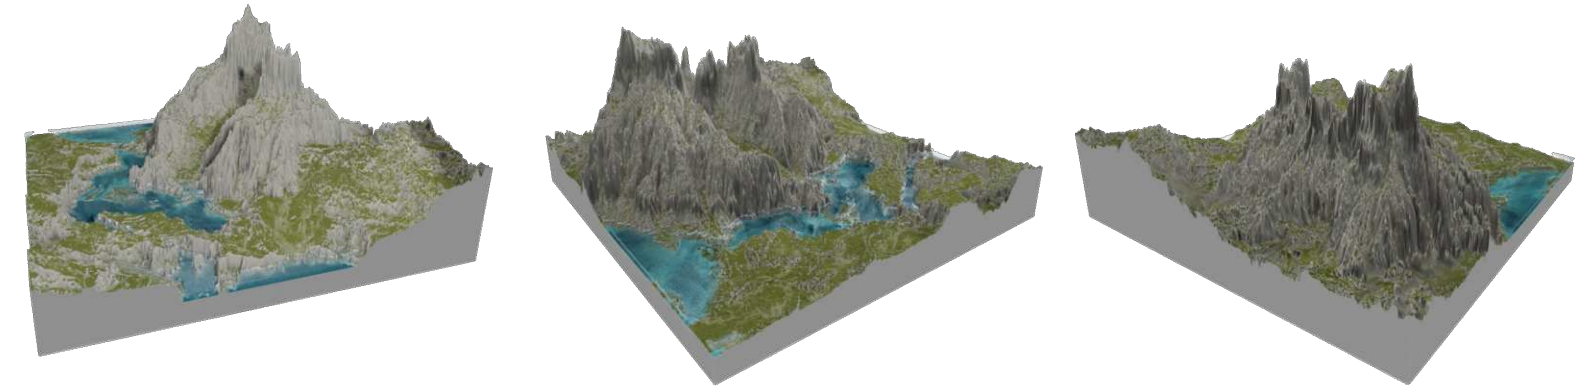

Stone Arch

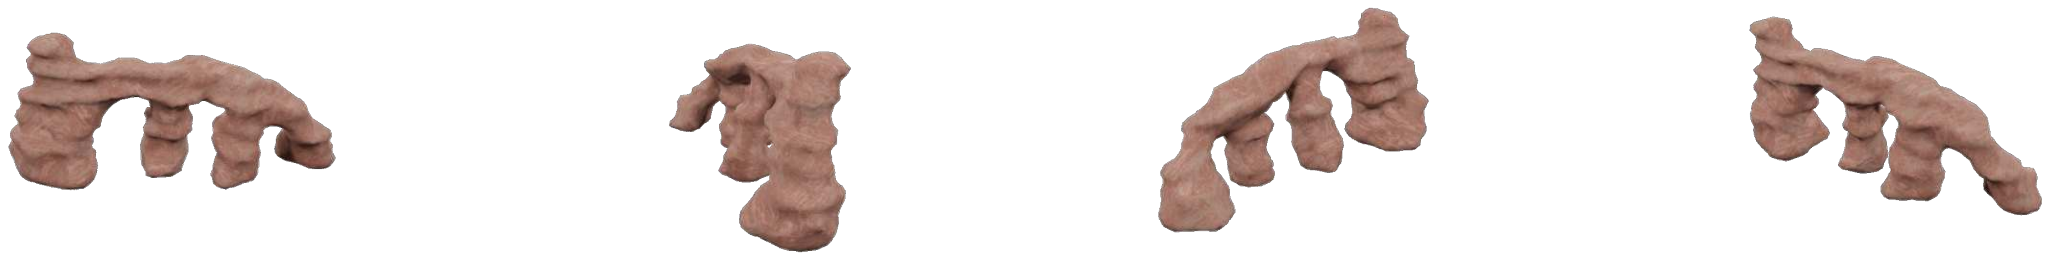

Stone Sculpture

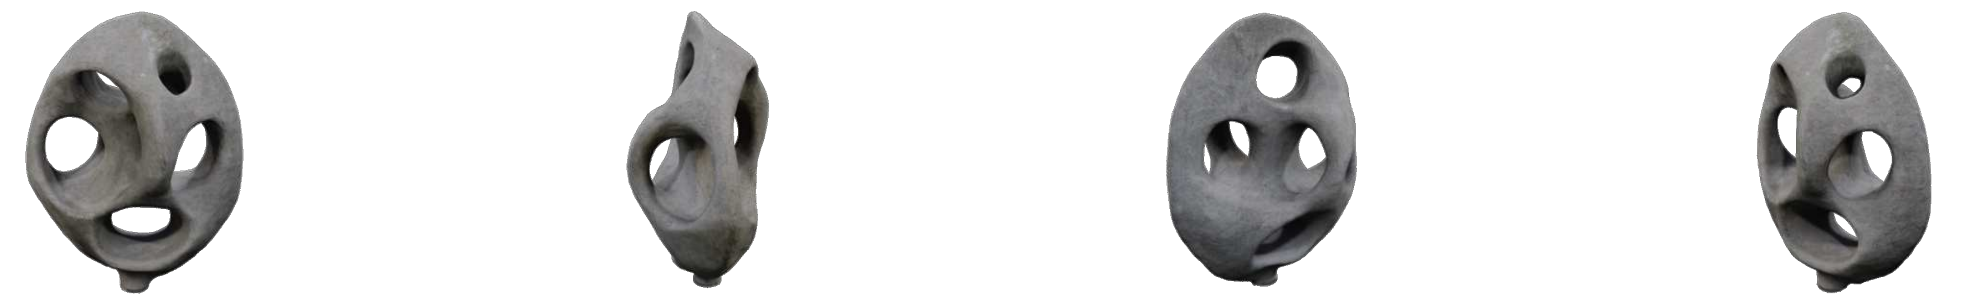

St Alphage

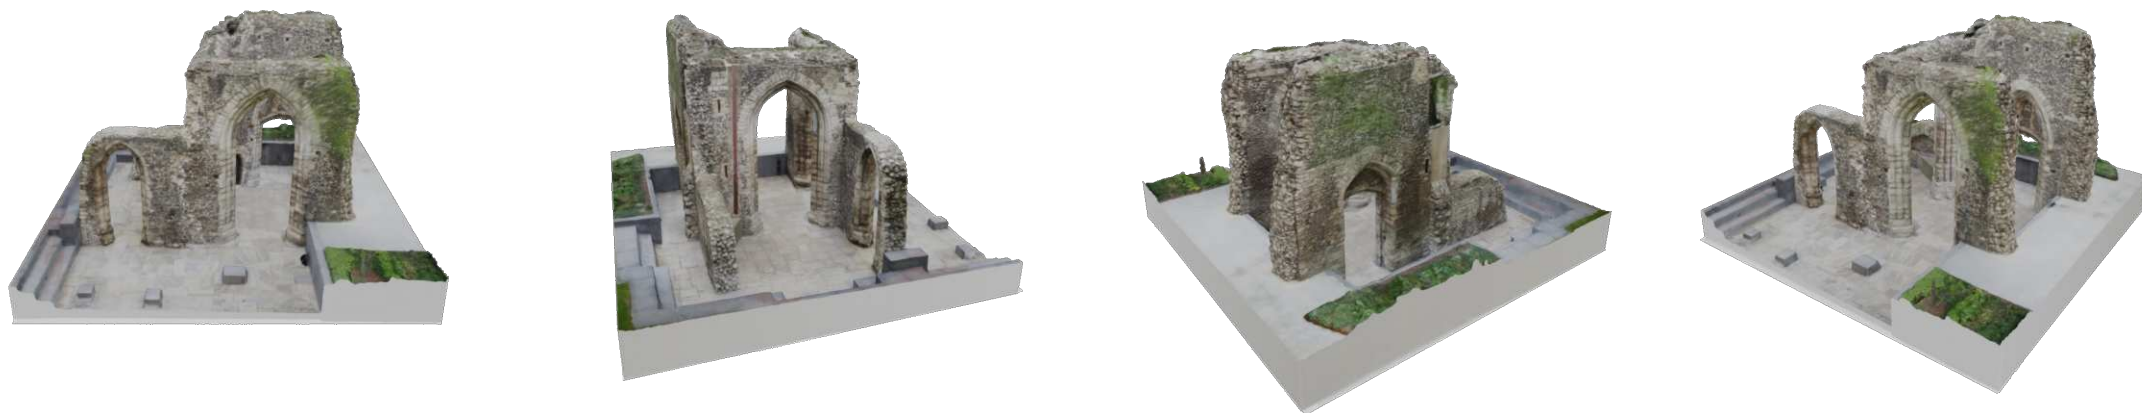

Stylized Cactus

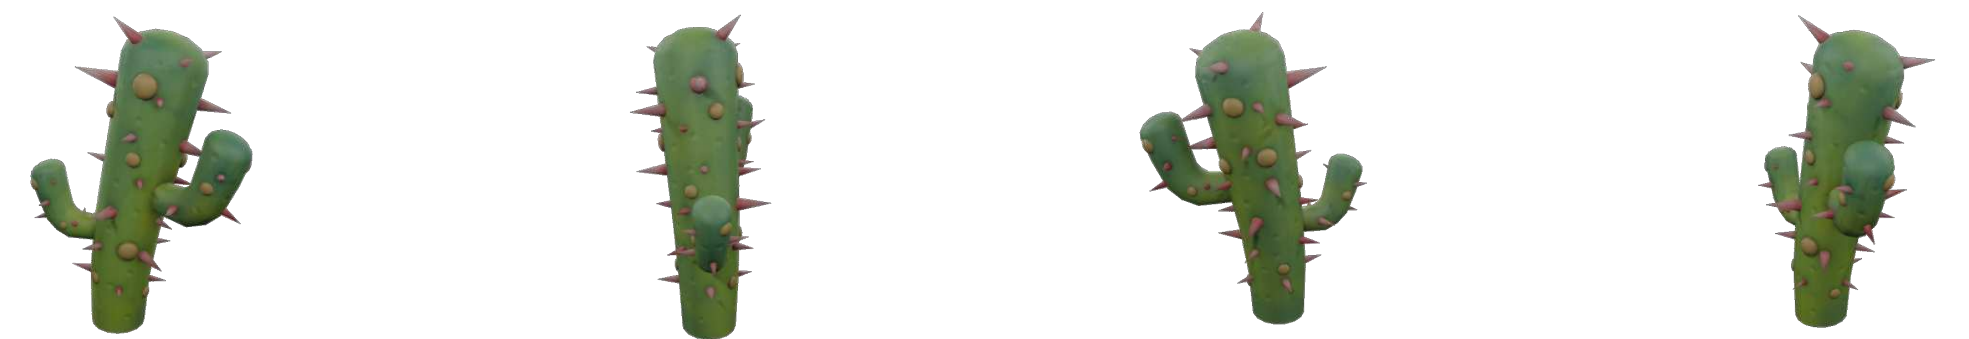

Spinsters Rock

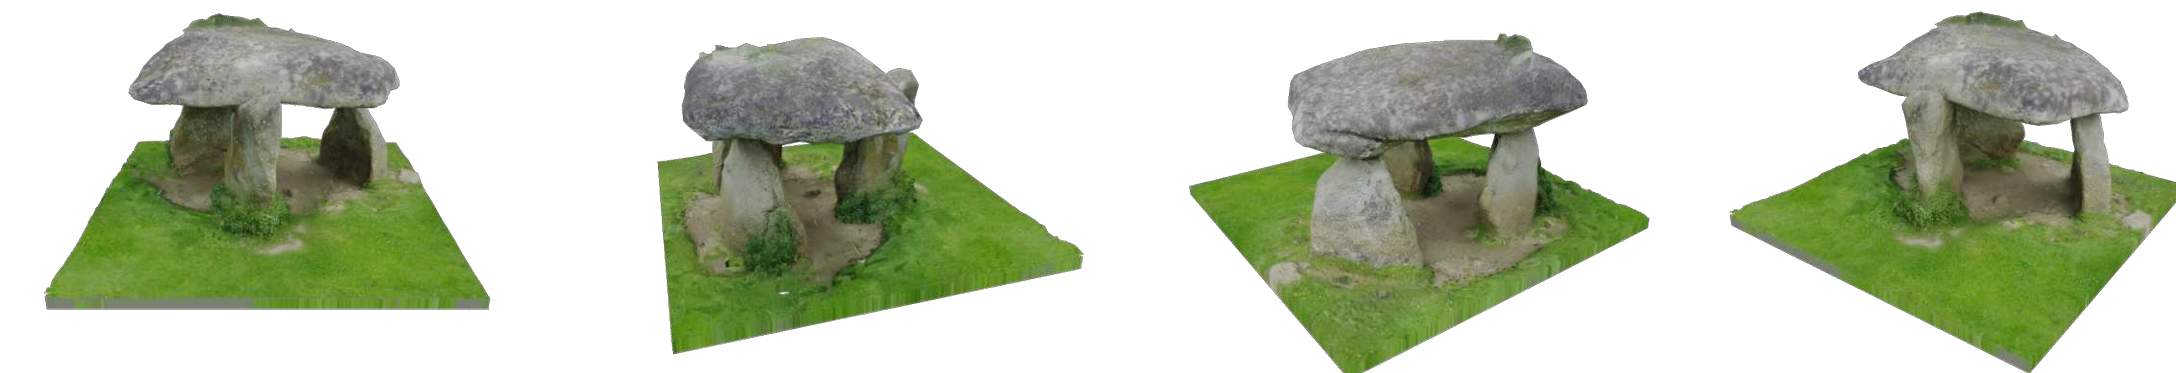

The Devil's Tower

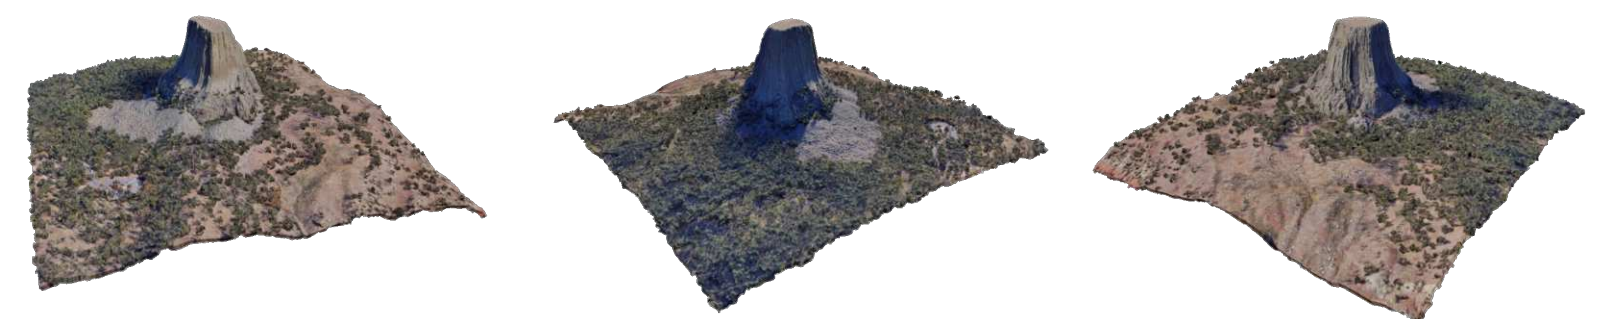

The Vast Land

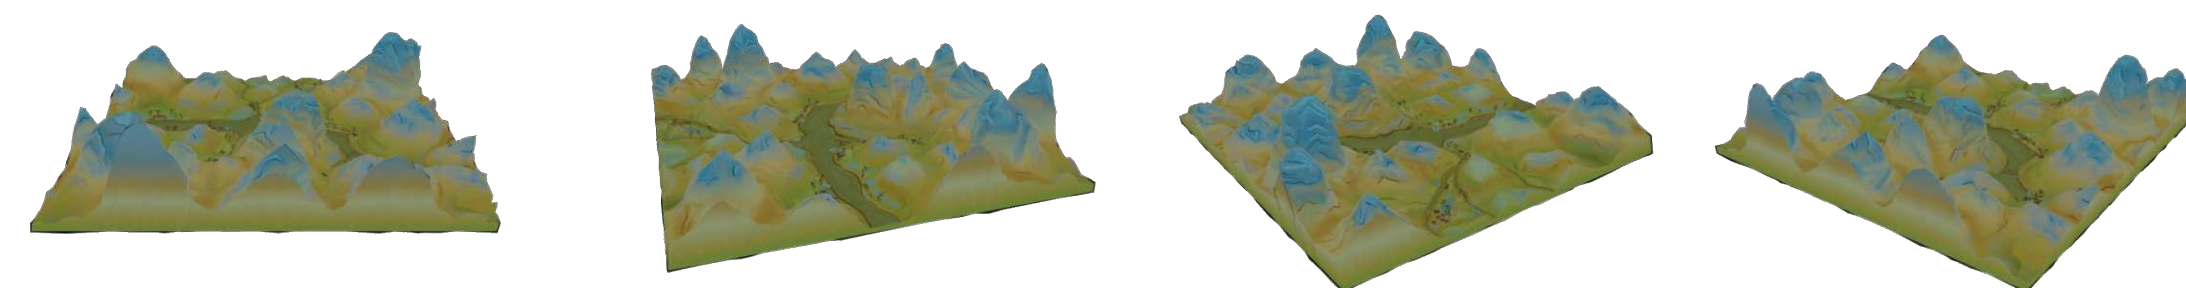

Volcano Island Lowpoly

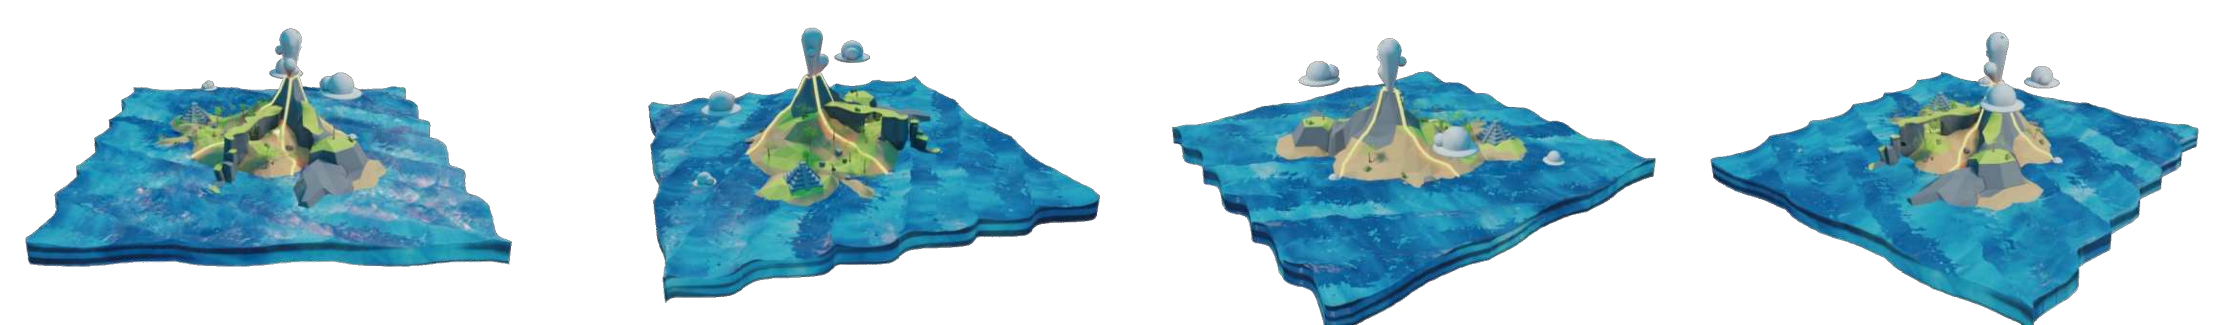



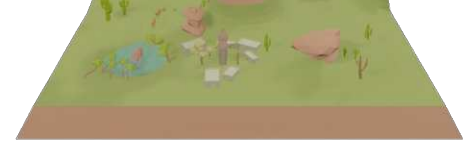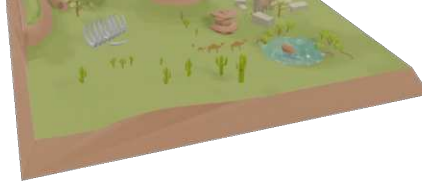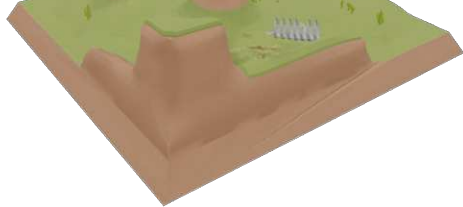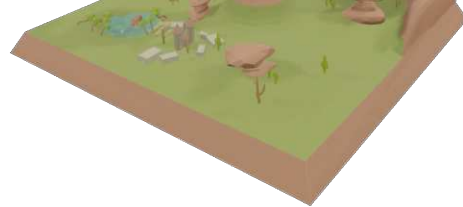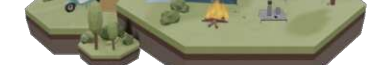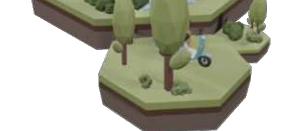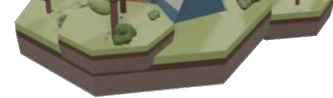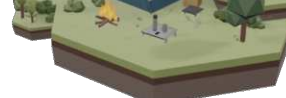

Spinsters Rock

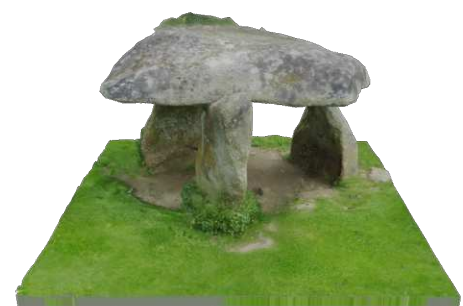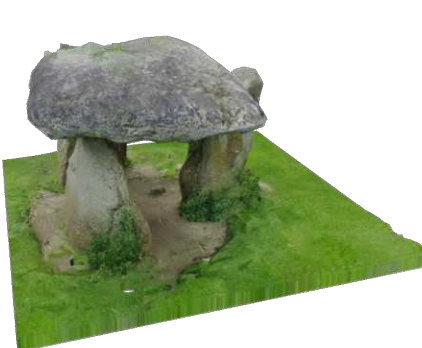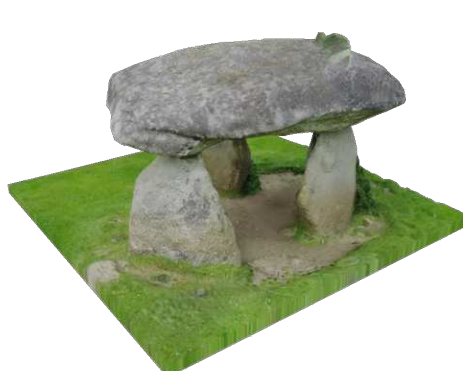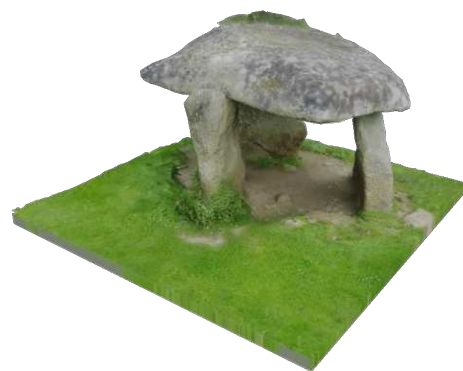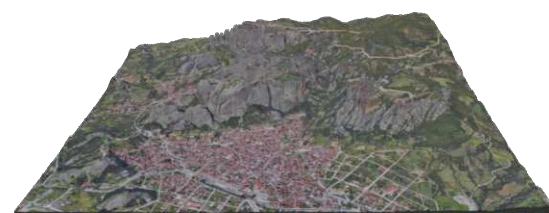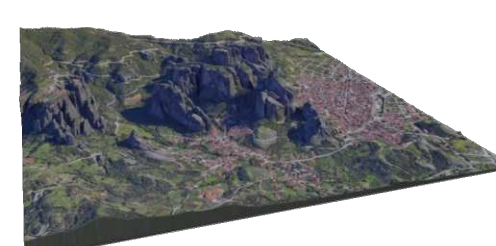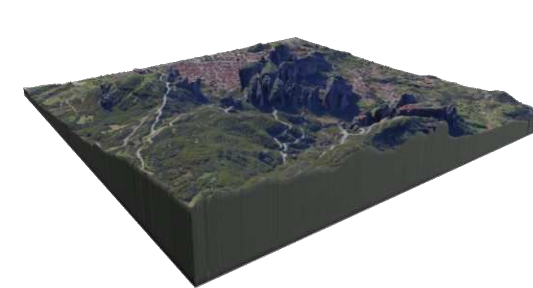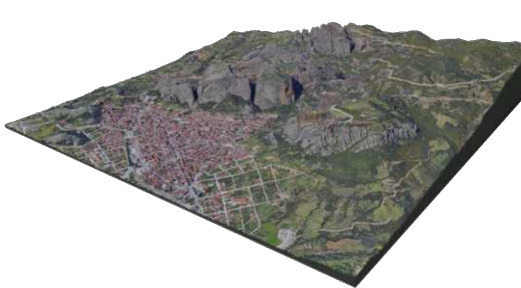

Meteora

Volcano Island Lowpoly

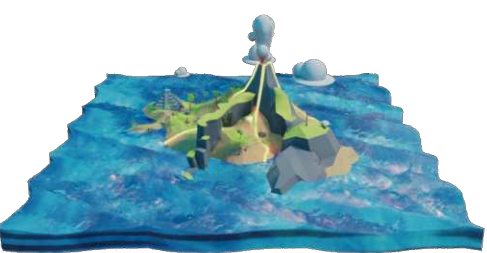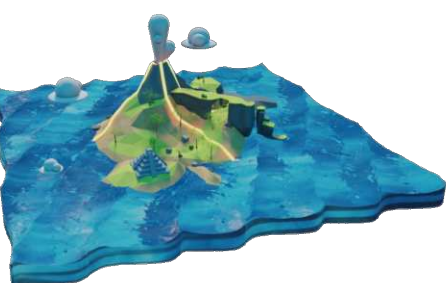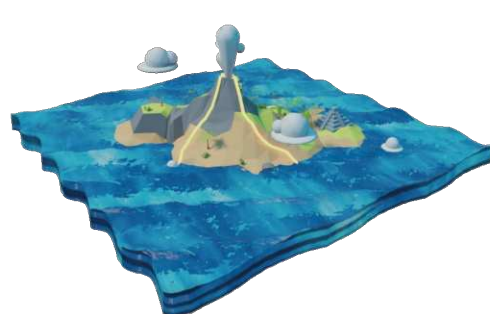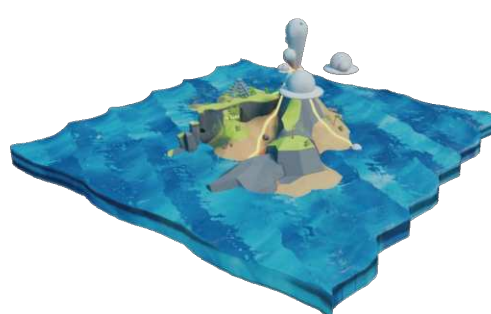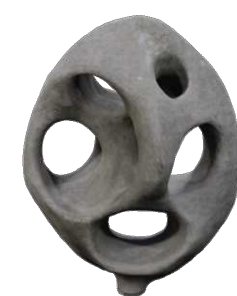

Stone Sculpture

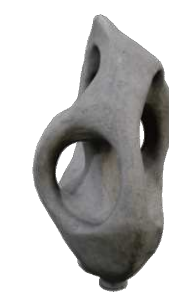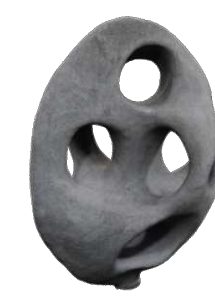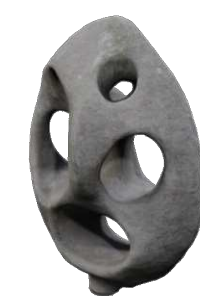

St Alphege

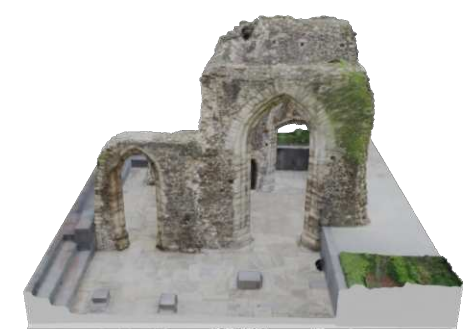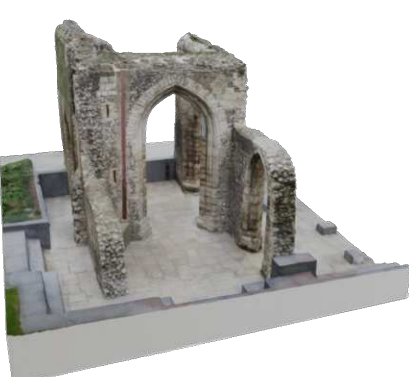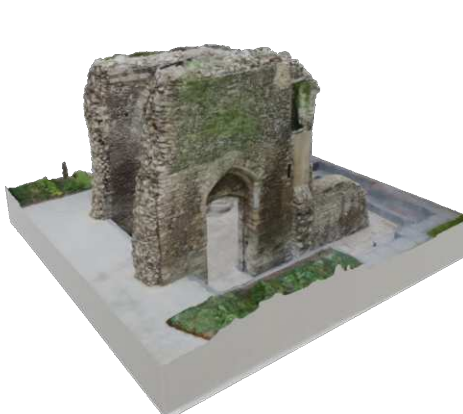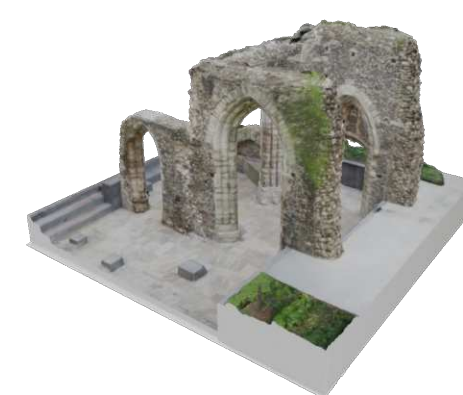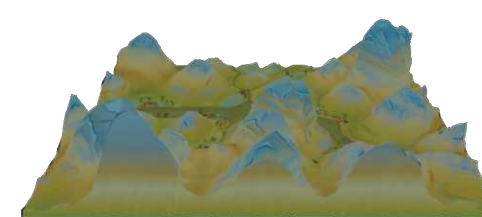

The Vast Land

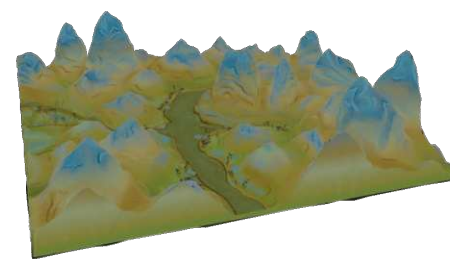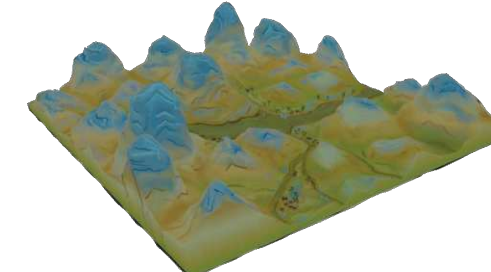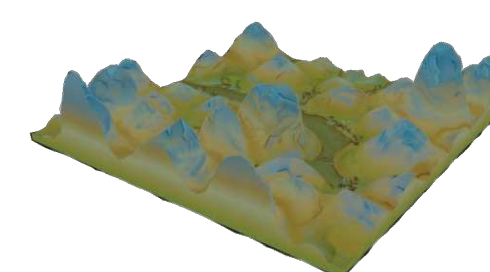

Green Island

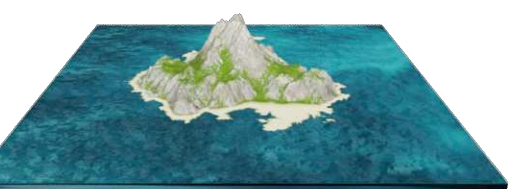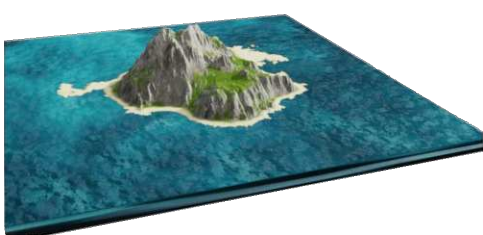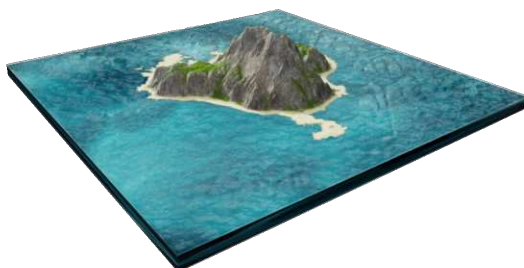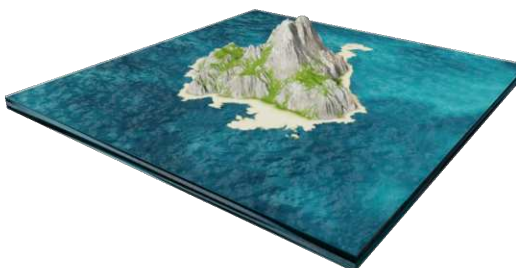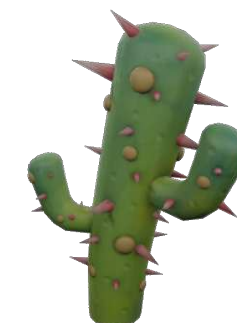

The Vast Land

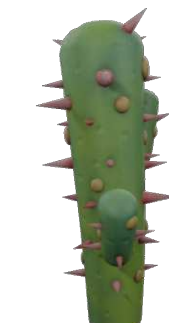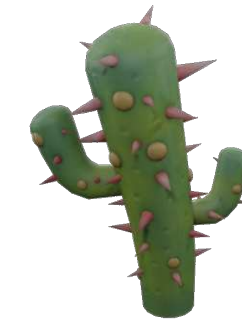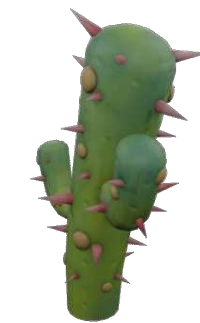

Mountain

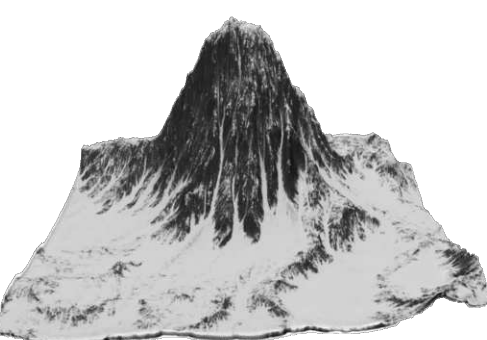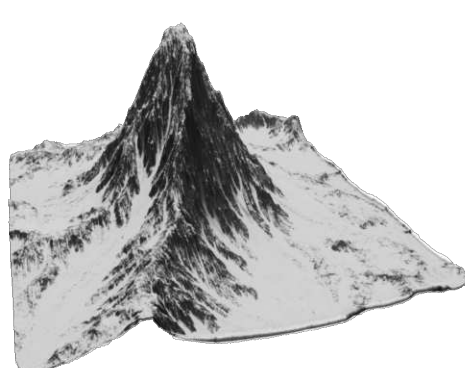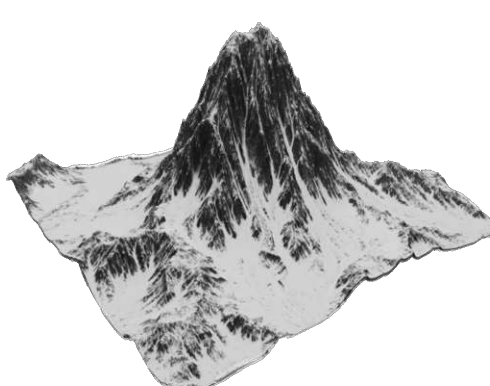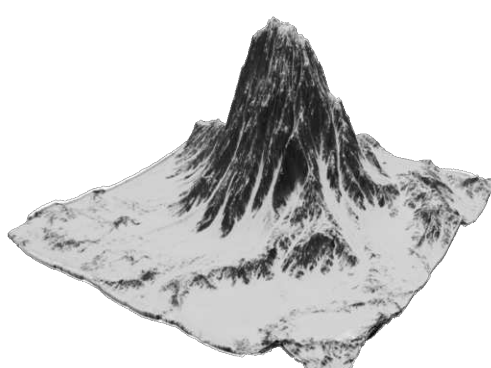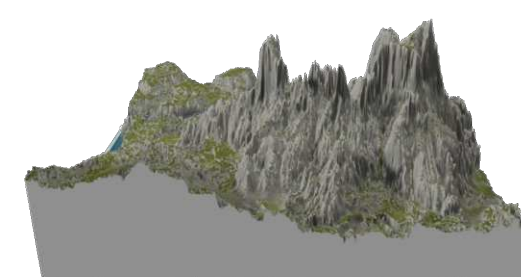

Mountain with Lakes

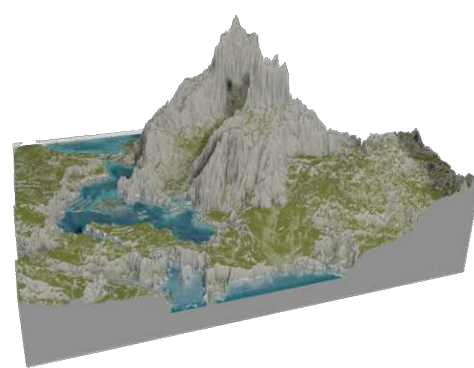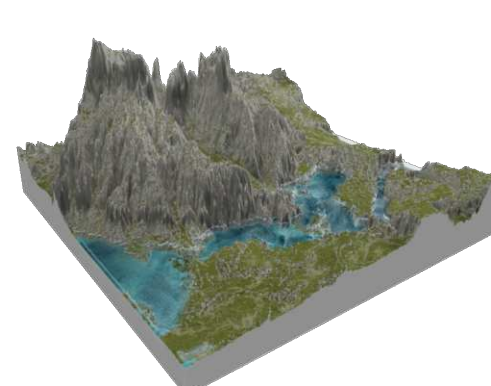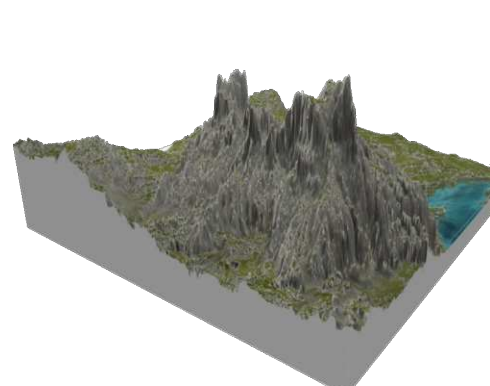

The Devil's Tower

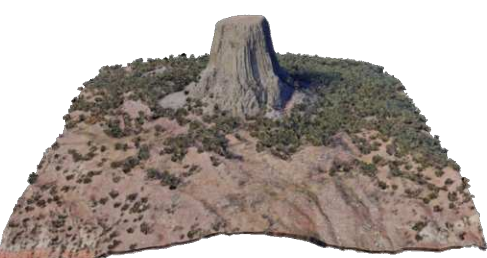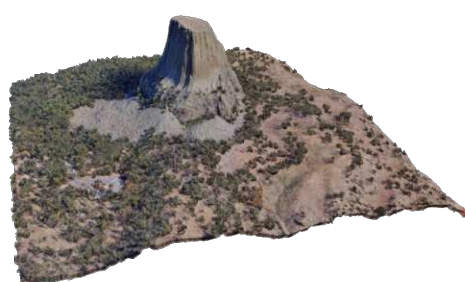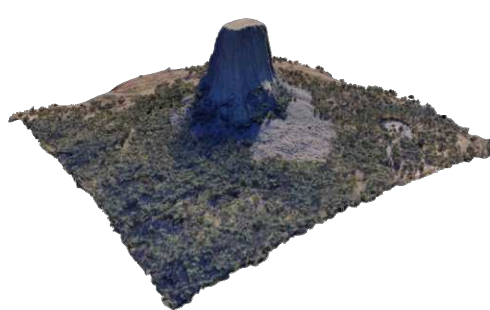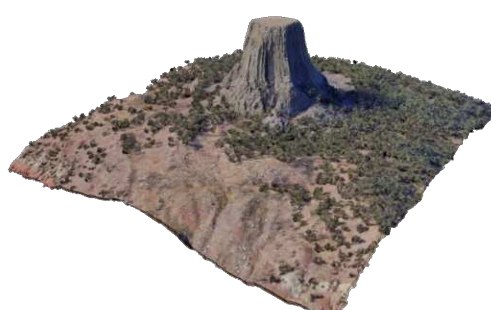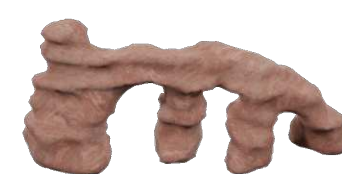

Stone Arch

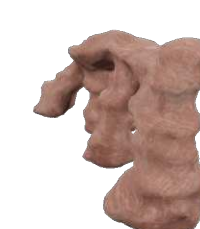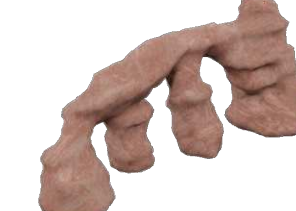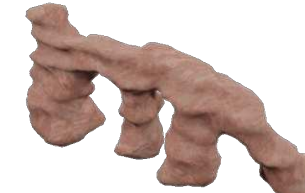

Calda House

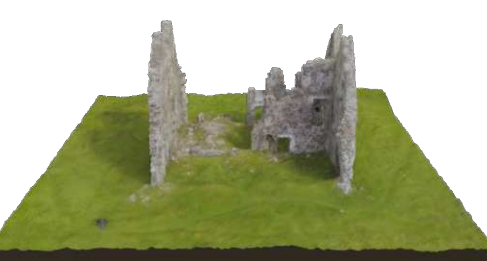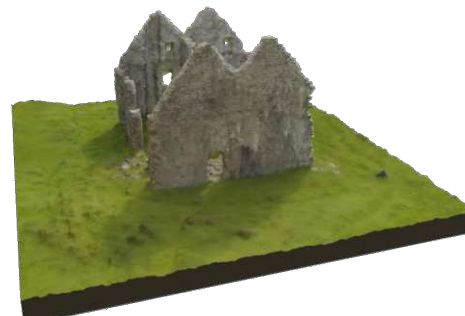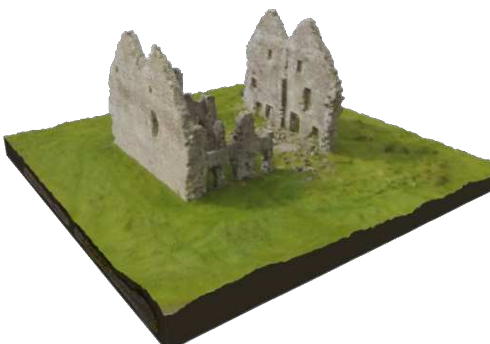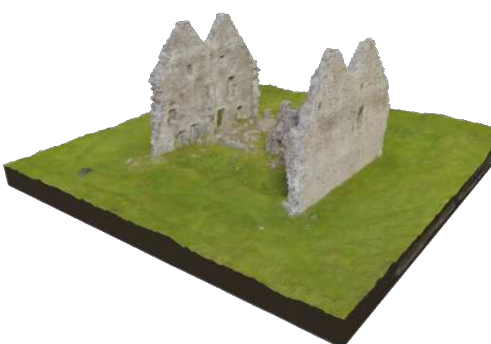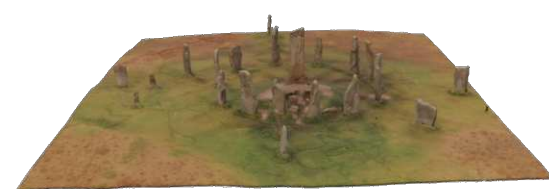

Callanish

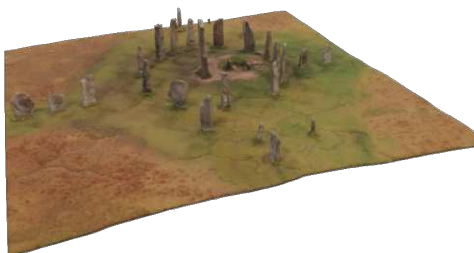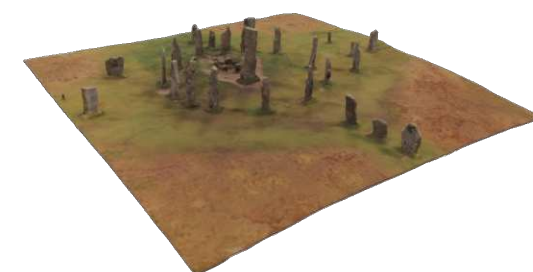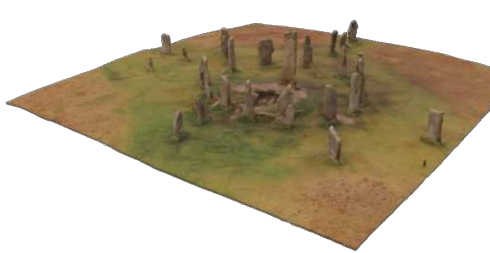

Cactus Cereus

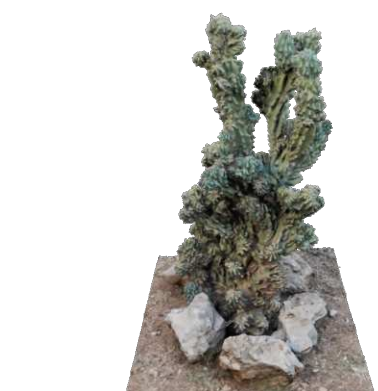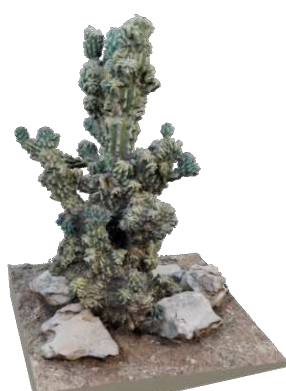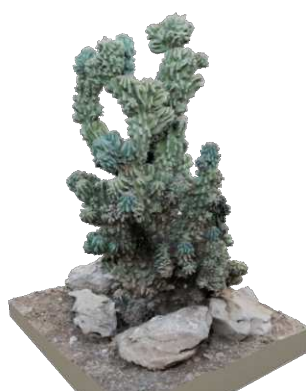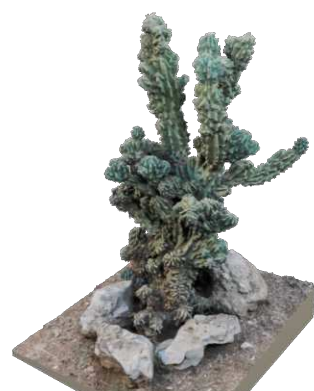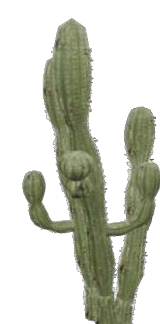

Cactus Saguaro

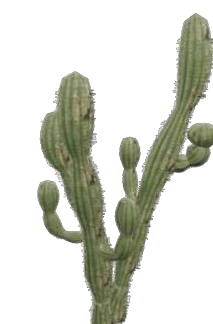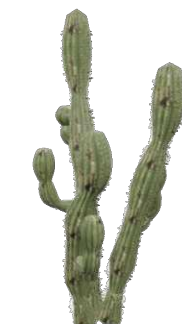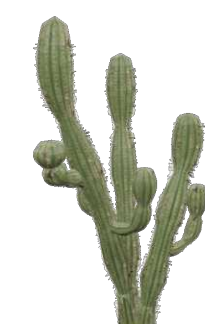

Supplement: Supplementary file 2 [file supplementary_exemplar.pdf]
