# Supplementary material for: Patch-based 3D Natural Scene Generation from a Single Example
Source: arXiv:2304.12670 source file (2023-04-26)
Supplement: Supplementary file 3 [file supplementary_r_effects.pdf]

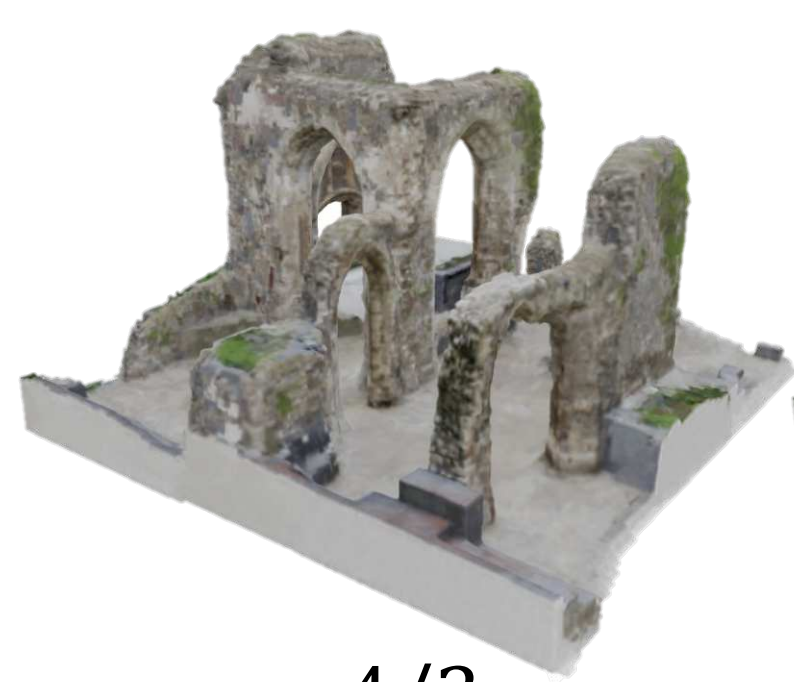

$$r = 4/3$$

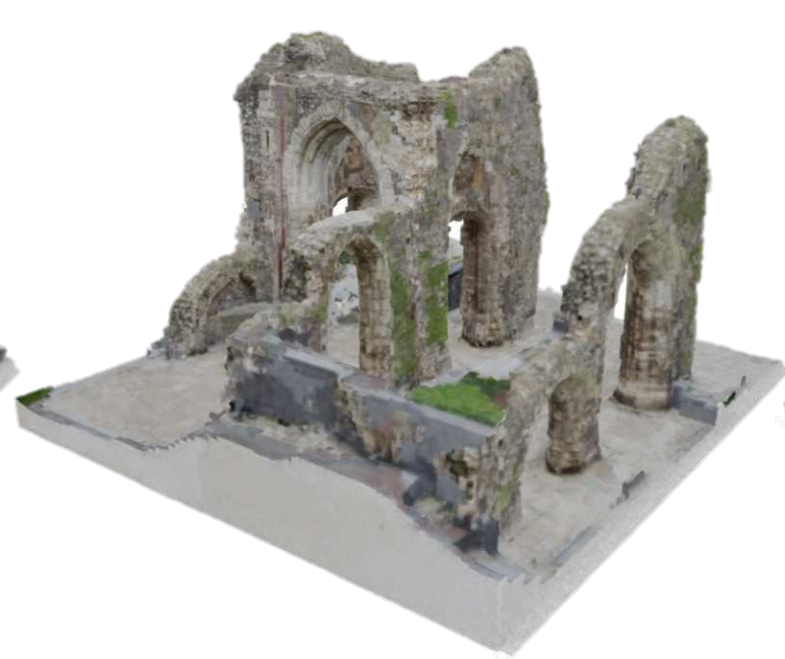

$$r = 5/3$$

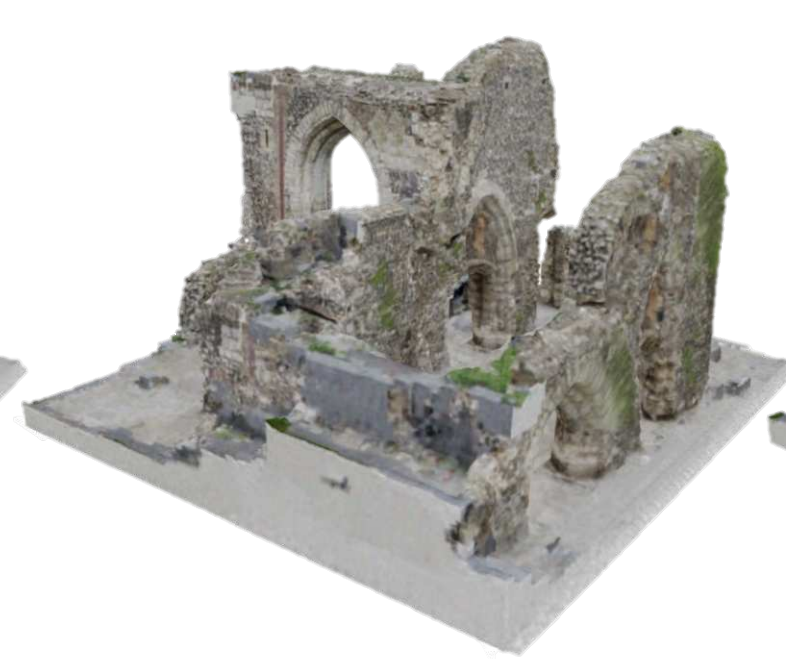

$$r = 6/3$$

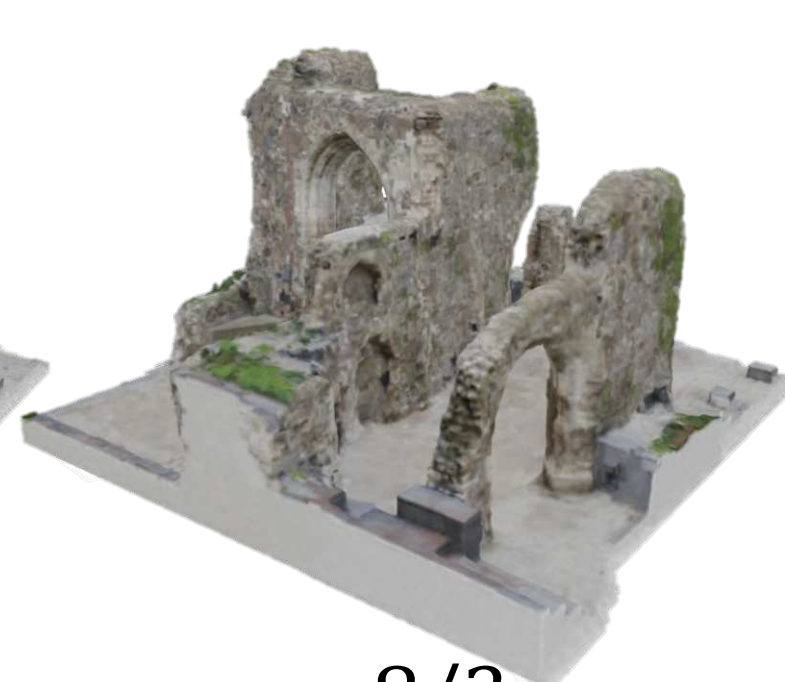

$$r = 8/3$$

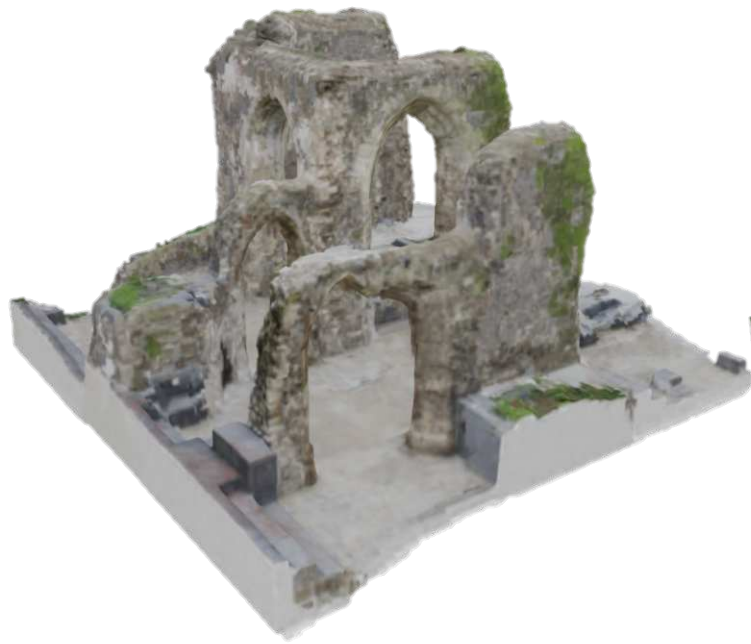

$$r = 4/3$$

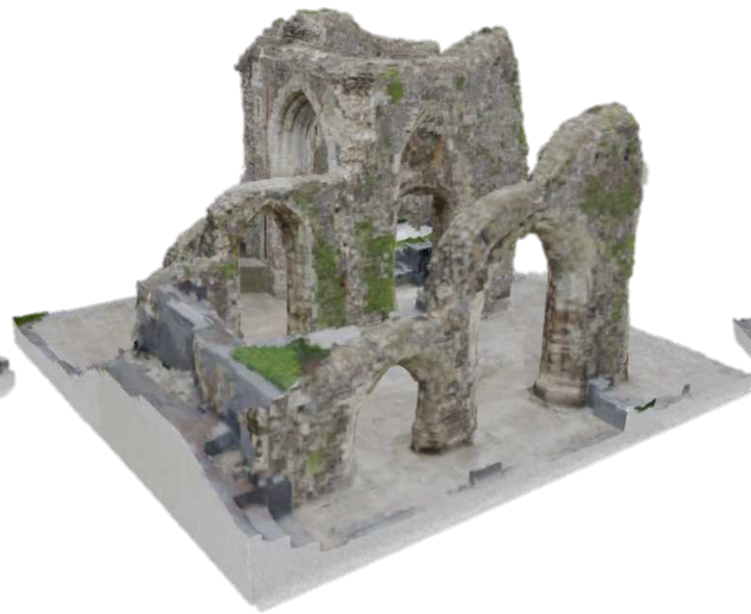

$$r = 5/3$$

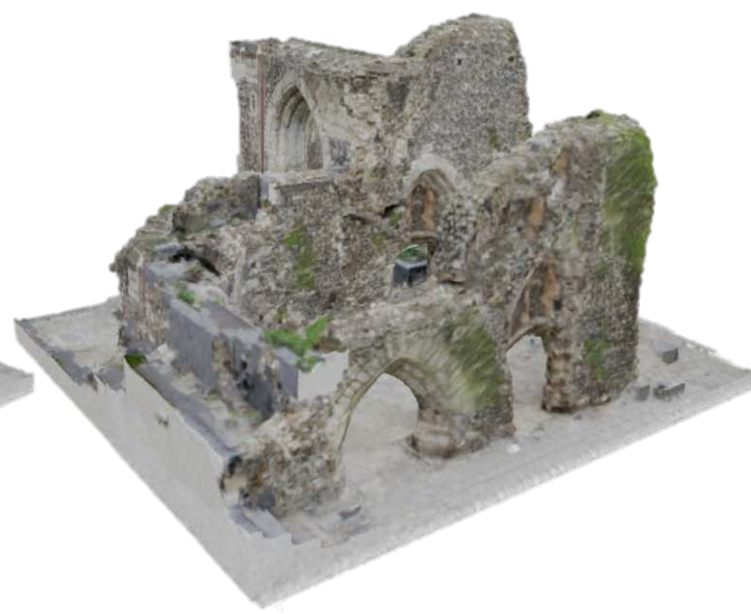

$$r = 6/3$$

$$r = 8/3$$

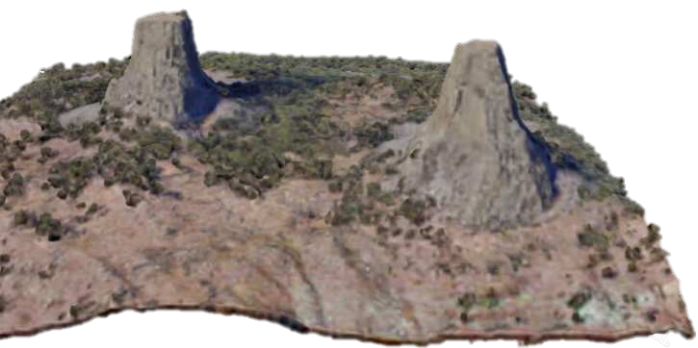

$$r = 4/3$$

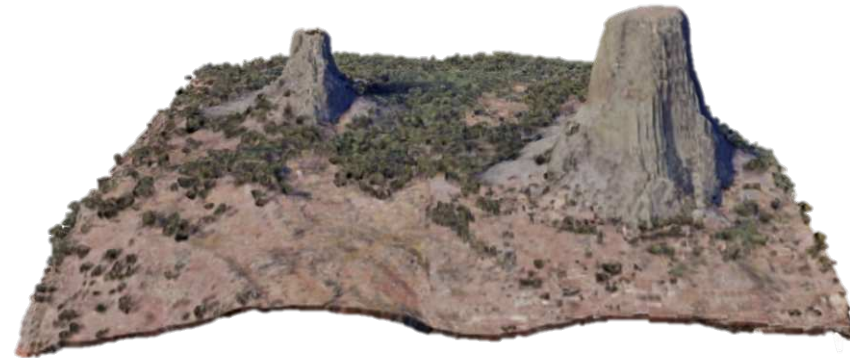

$$r = 5/3$$

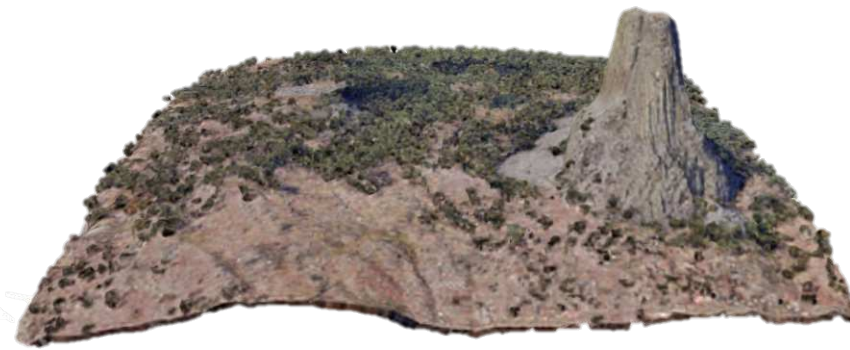

$$r = 6/3$$

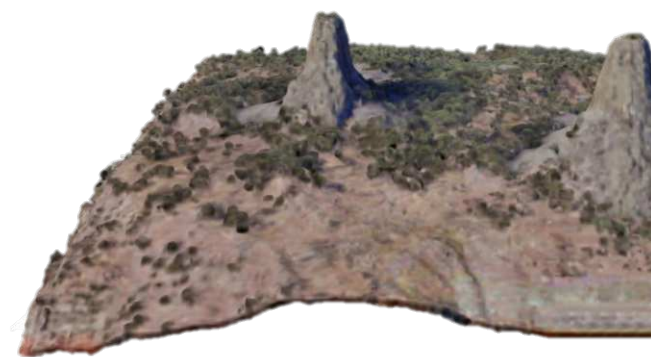

$$r = 8/3$$
