# Supplementary material for: Patch-based 3D Natural Scene Generation from a Single Example
Source: arXiv:2304.12670 source file (2023-04-26)
Supplement: Supplementary file 4 [file supplementary_s_0_effects.pdf]

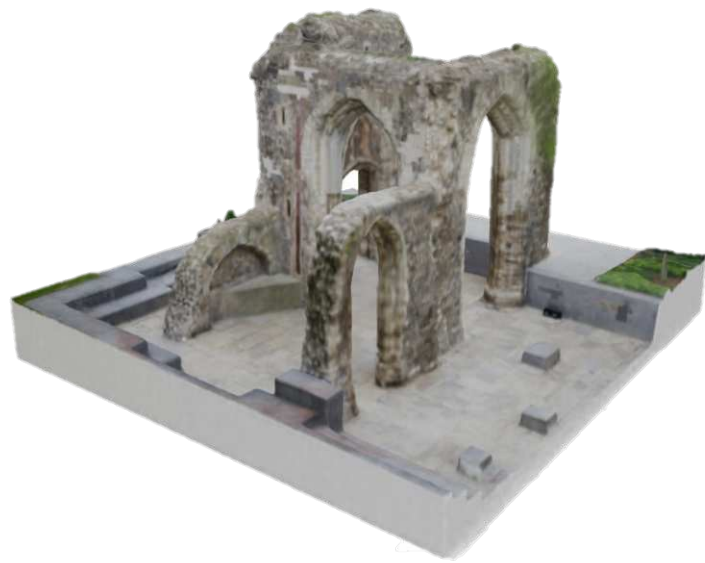

$Reso(S_0) = 12$

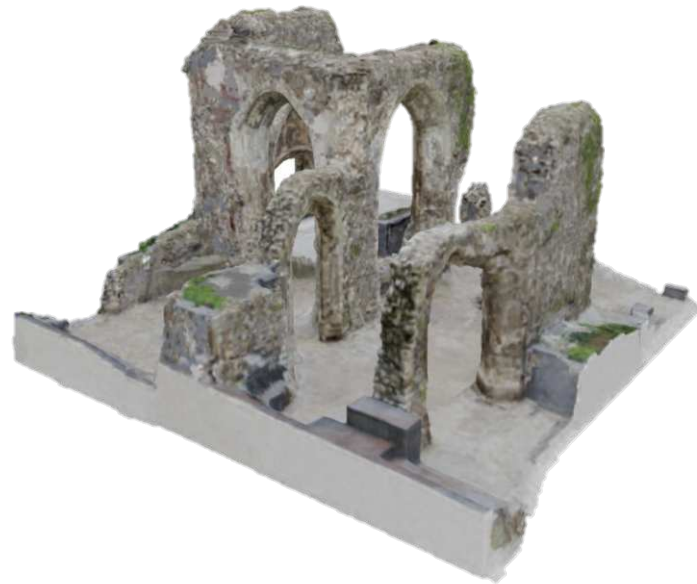

$Reso(S_0) = 16$

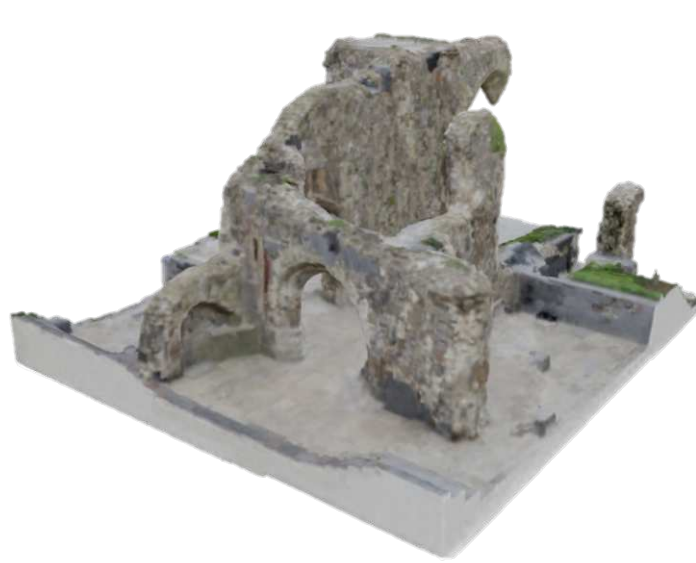

$Reso(S_0) = 21$

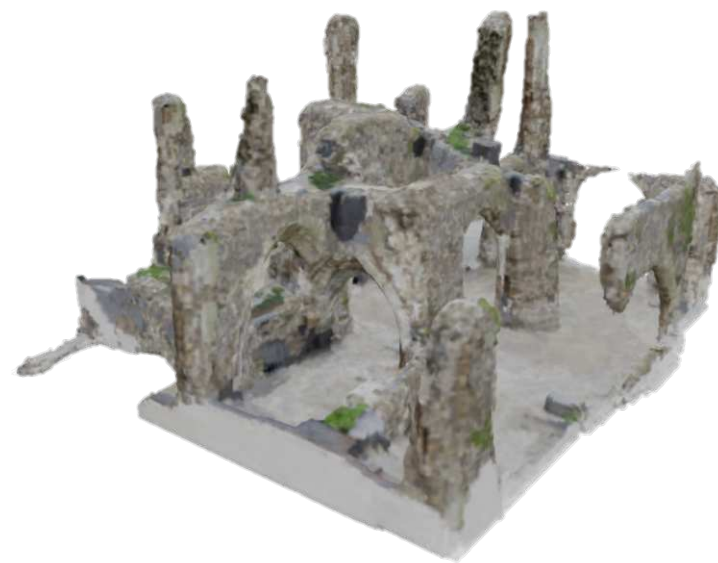

$Reso(S_0) = 28$

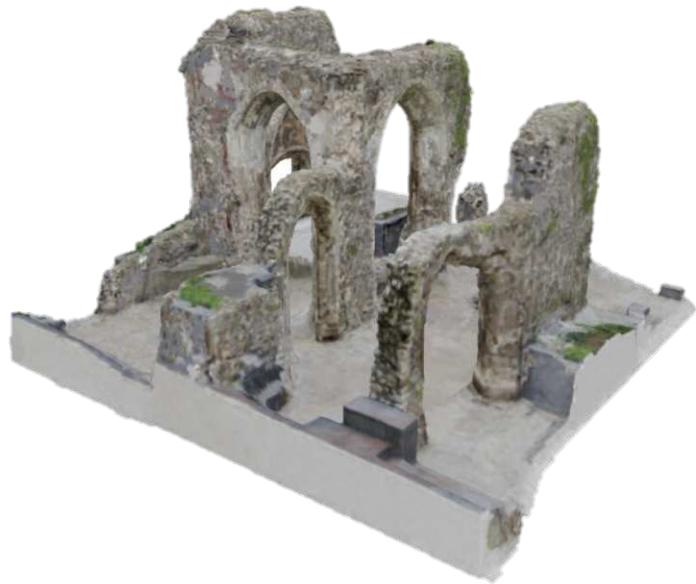

$Reso(S_0) = 16$

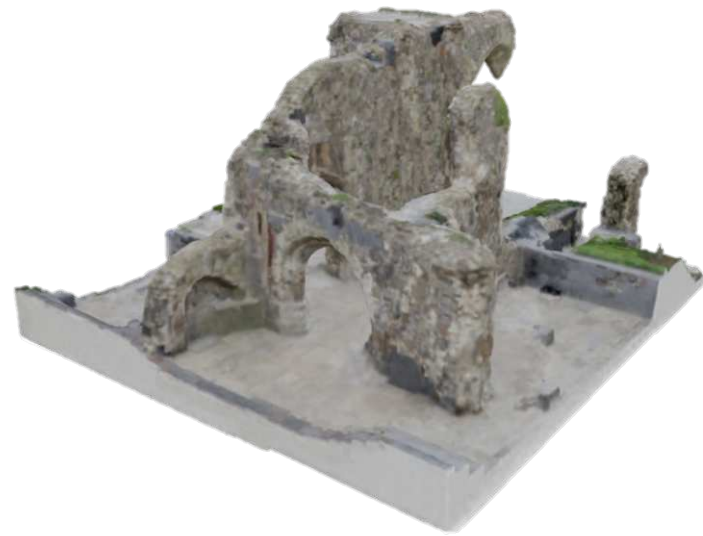

$Reso(S_0) = 21$

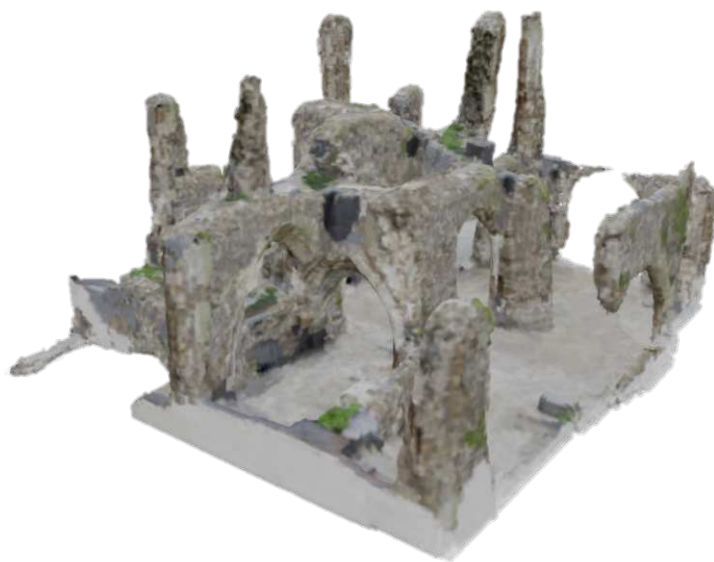

$Reso(S_0) = 28$

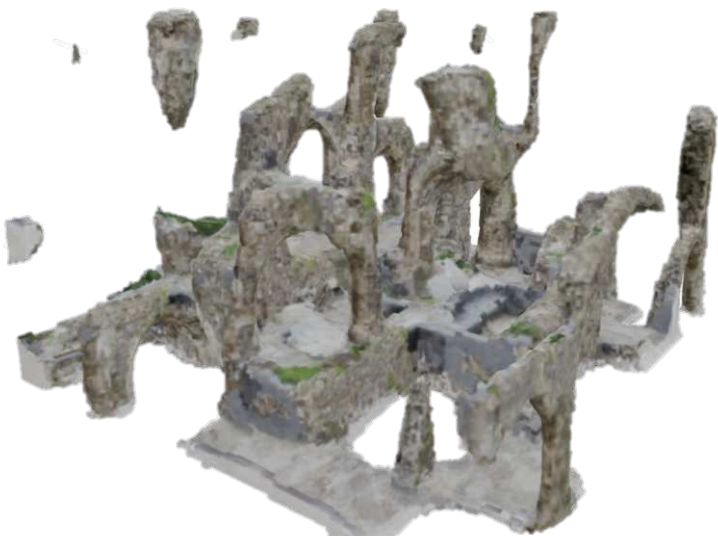

$Reso(S_0) = 38$
