# Supplementary material for: Patch-based 3D Natural Scene Generation from a Single Example
Source: arXiv:2304.12670 source file (2023-04-26)
Supplement: Supplementary file 5 [file supplementary_s_N_effects.pdf]

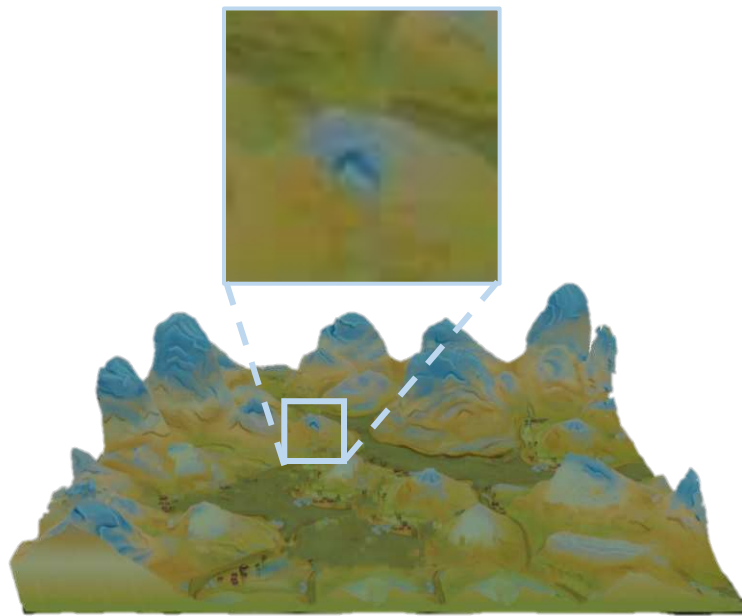

$Reso(S_N) = 121$

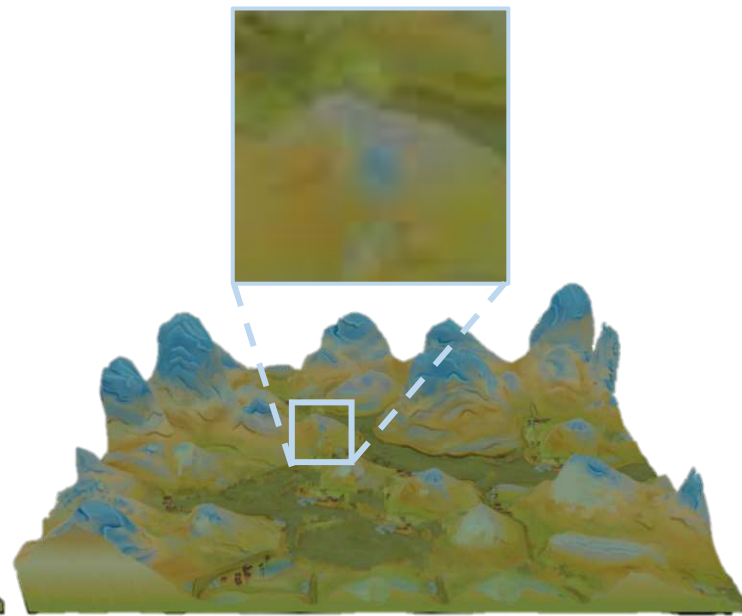

$Reso(S_N) = 162$

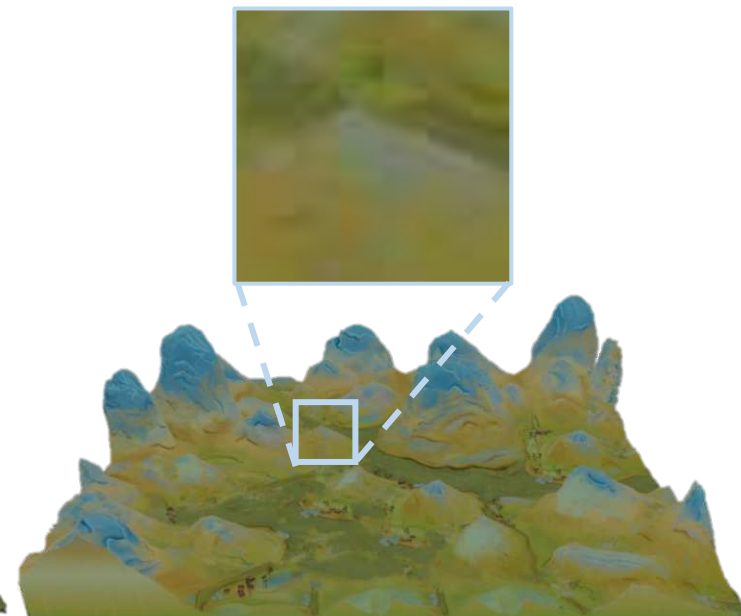

$Reso(S_N) = 216$

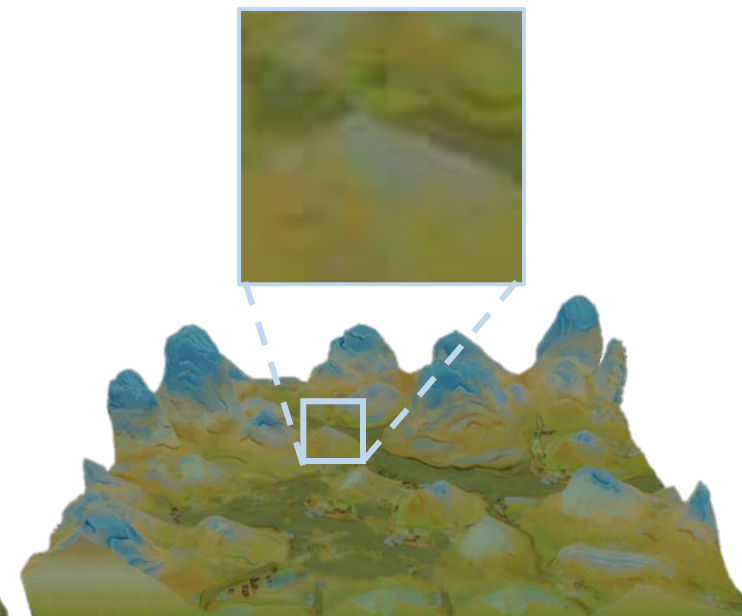

$Reso(S_N) = 288$

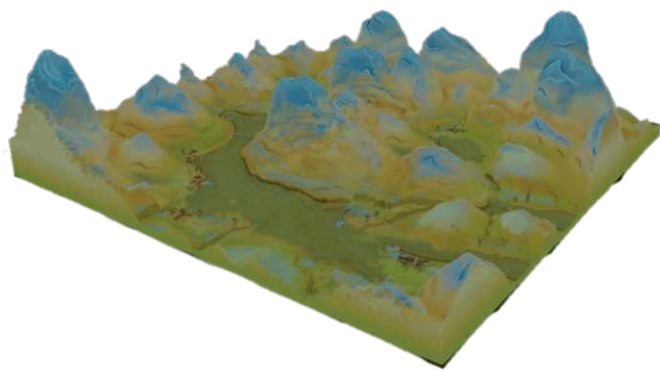

$Reso(S_N) = 121$

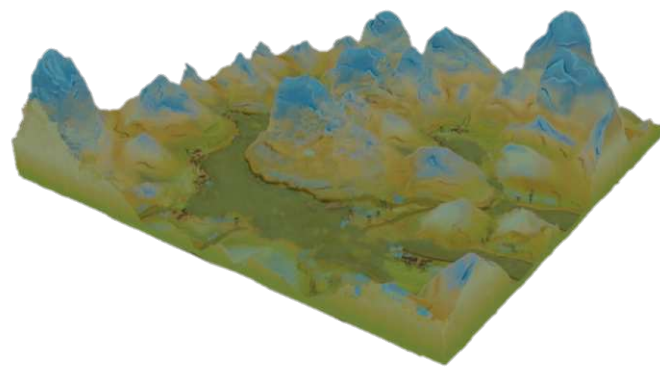

$Reso(S_N) = 162$

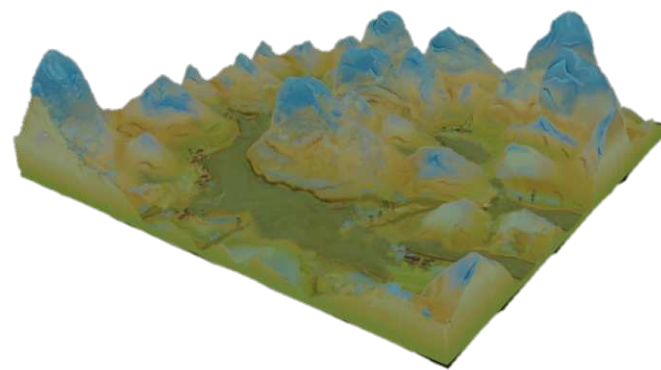

$Reso(S_N) = 216$

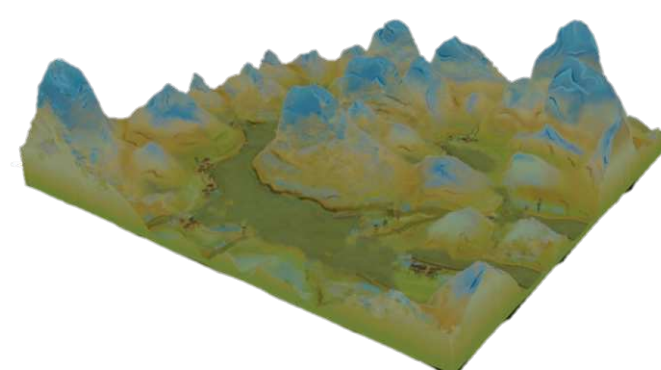

$Reso(S_N) = 288$
