# Supplementary material for: Patch-based 3D Natural Scene Generation from a Single Example
Source: arXiv:2304.12670 source file (2023-04-26)

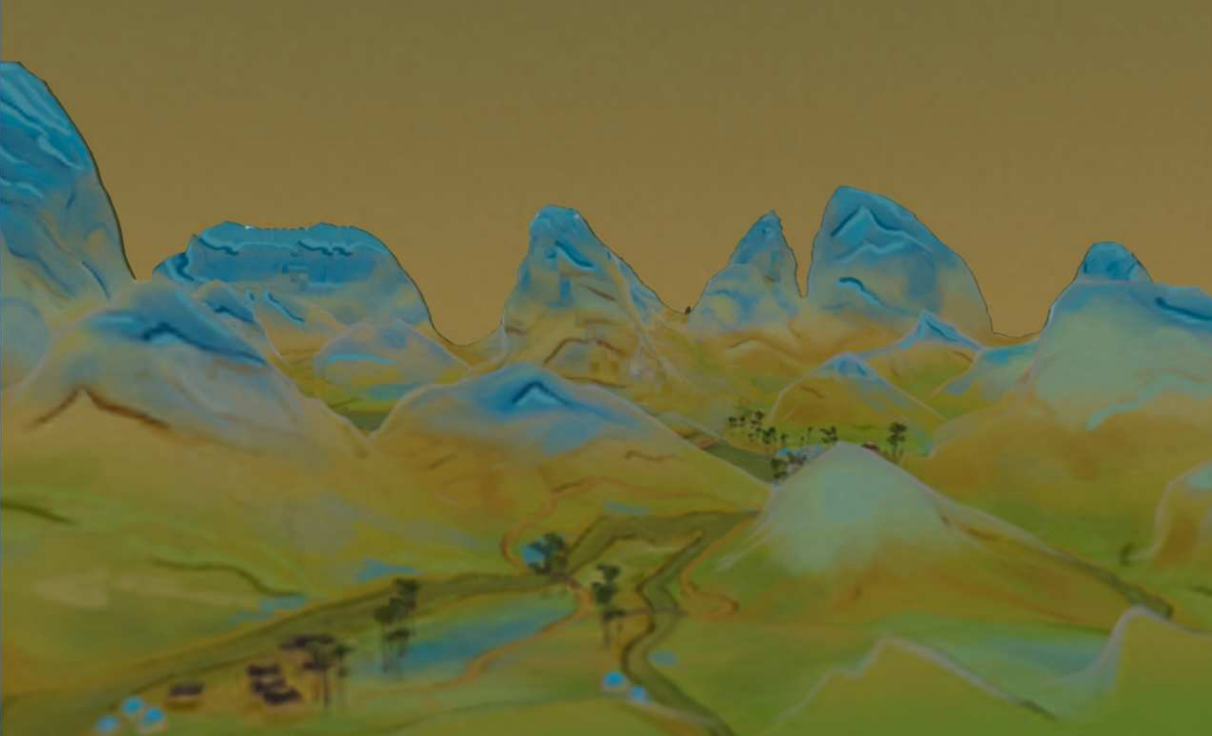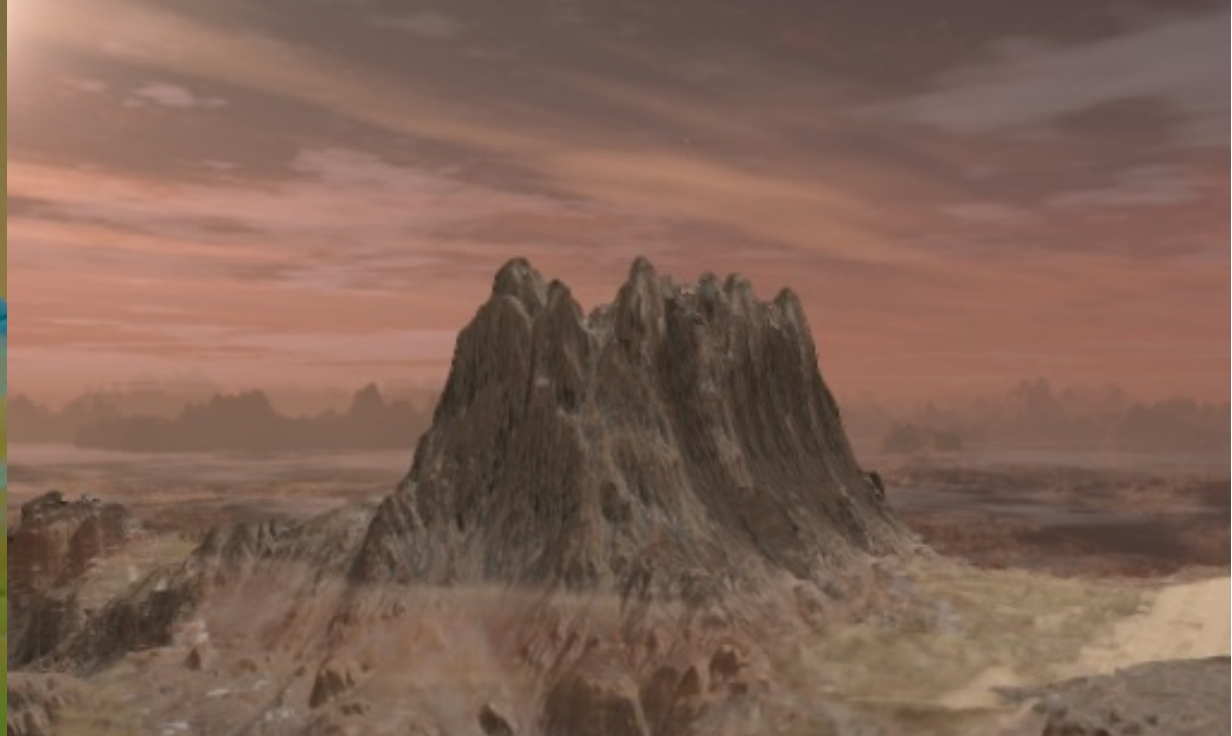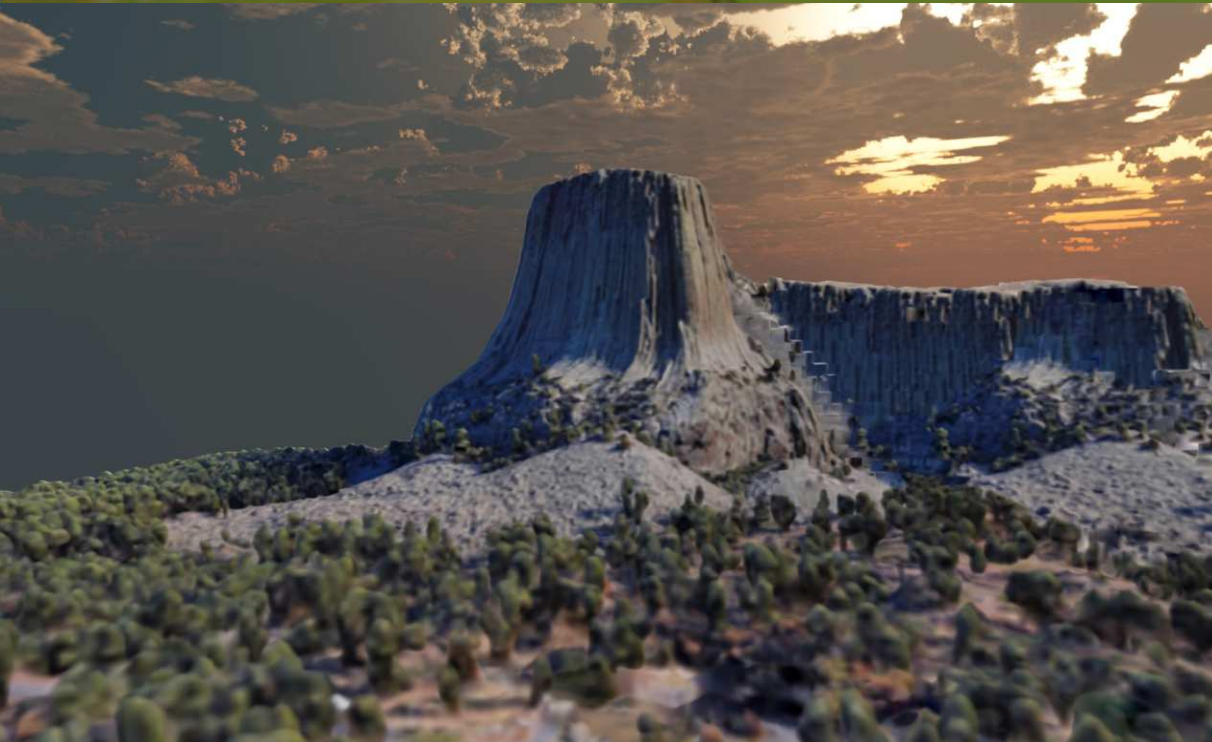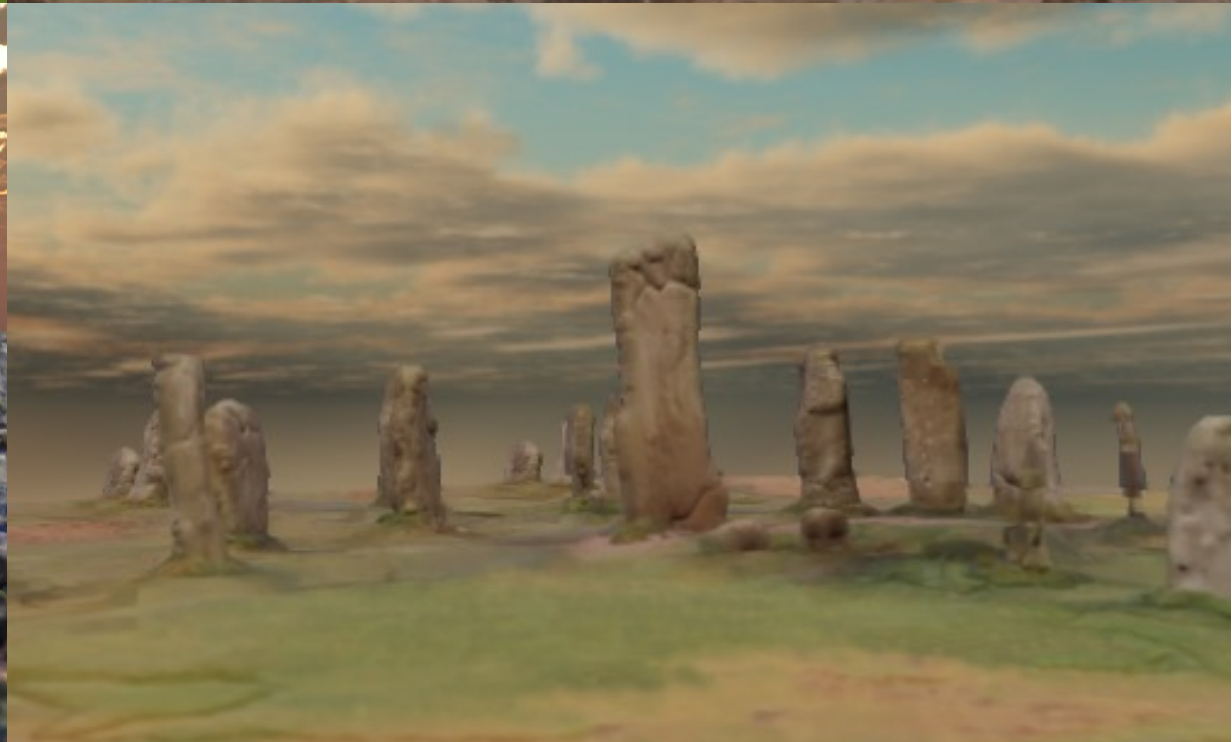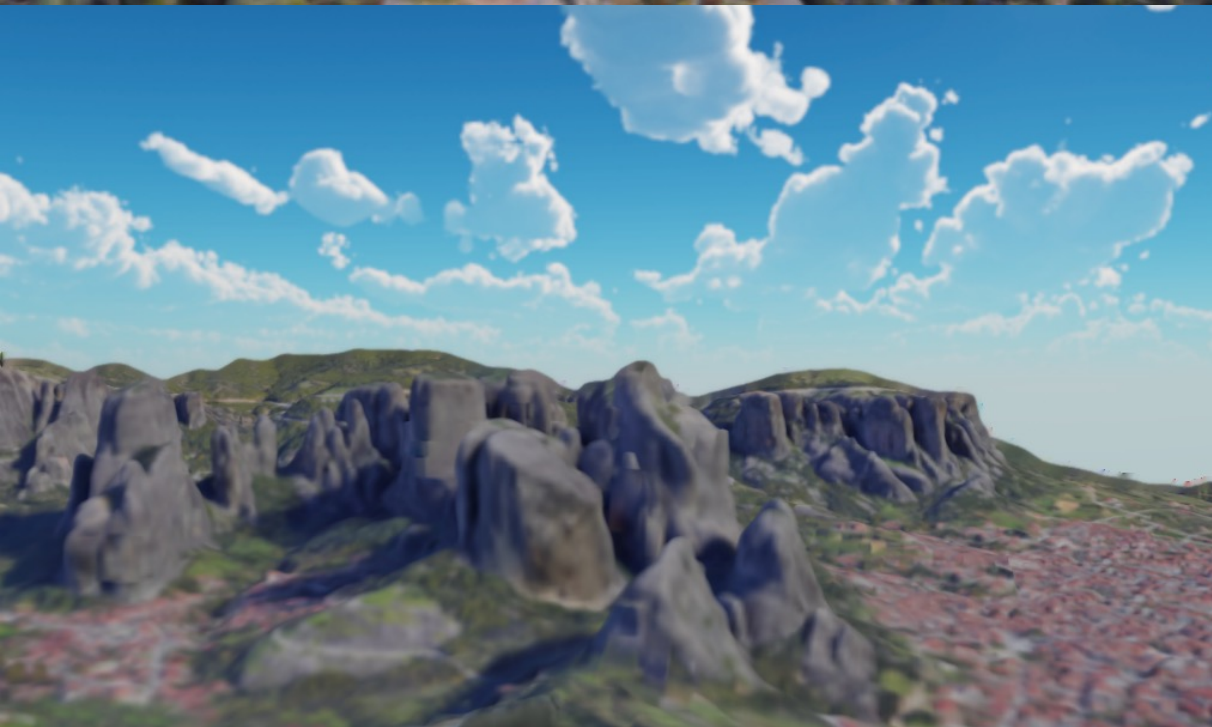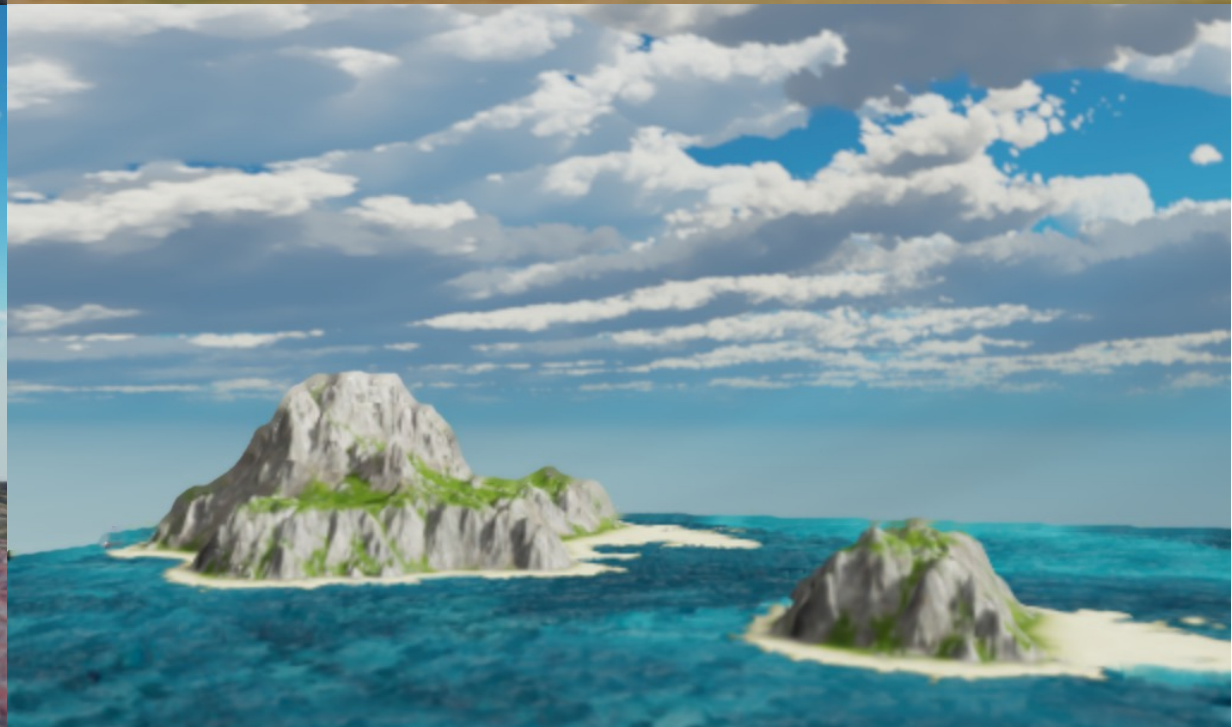



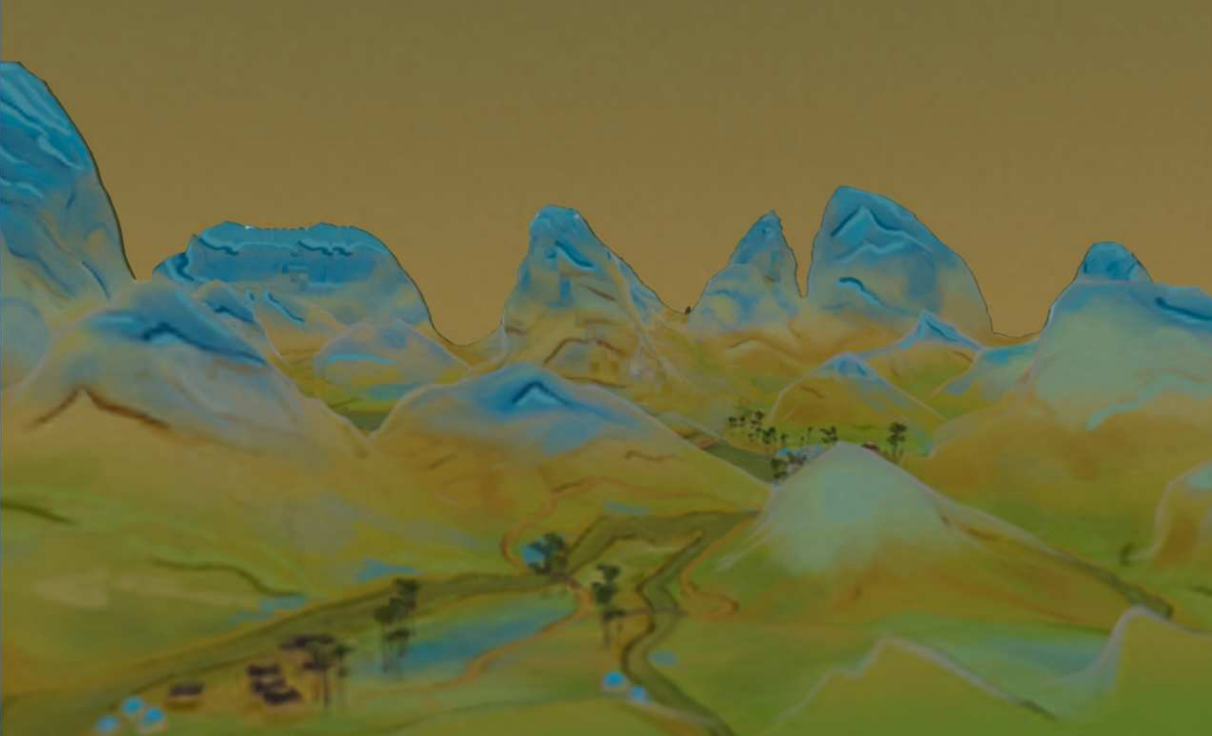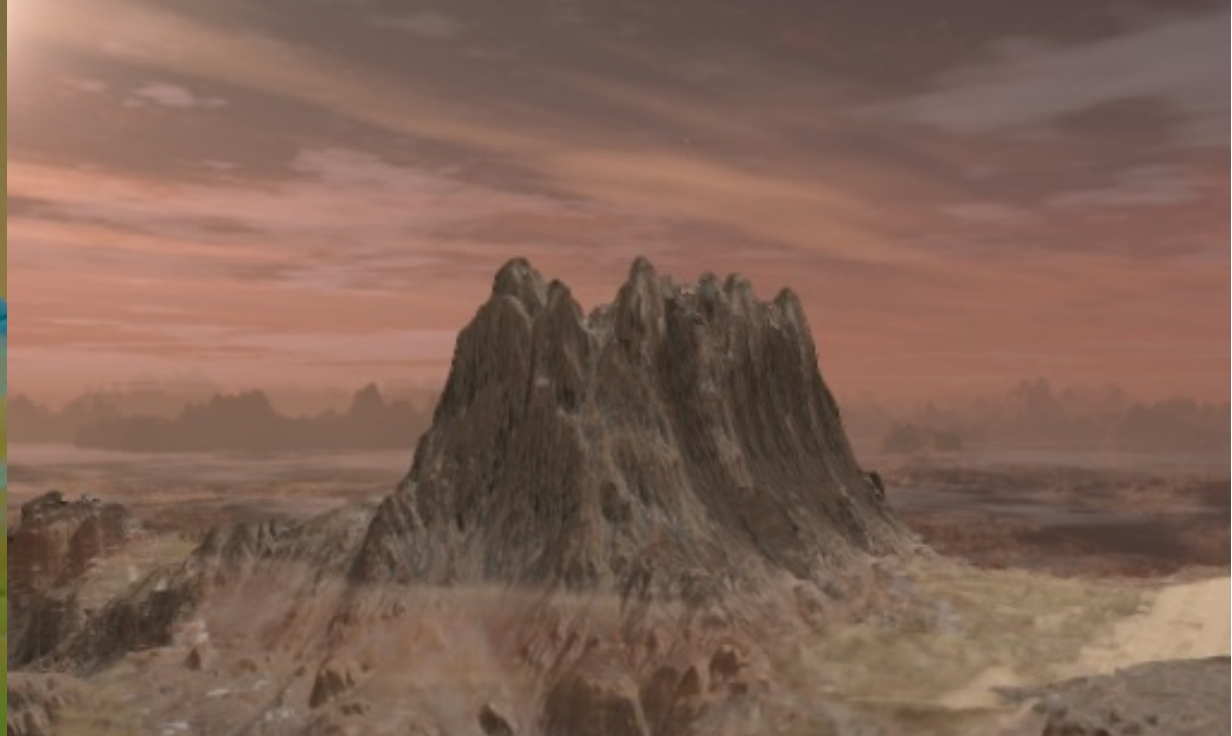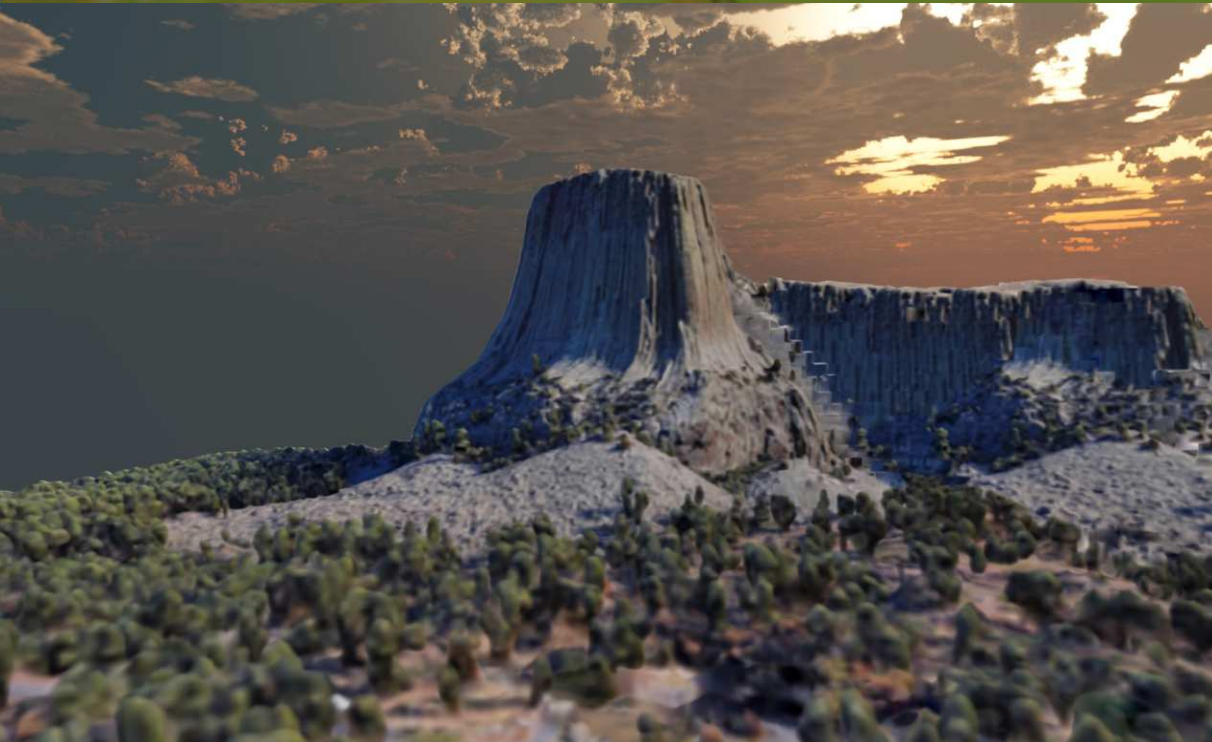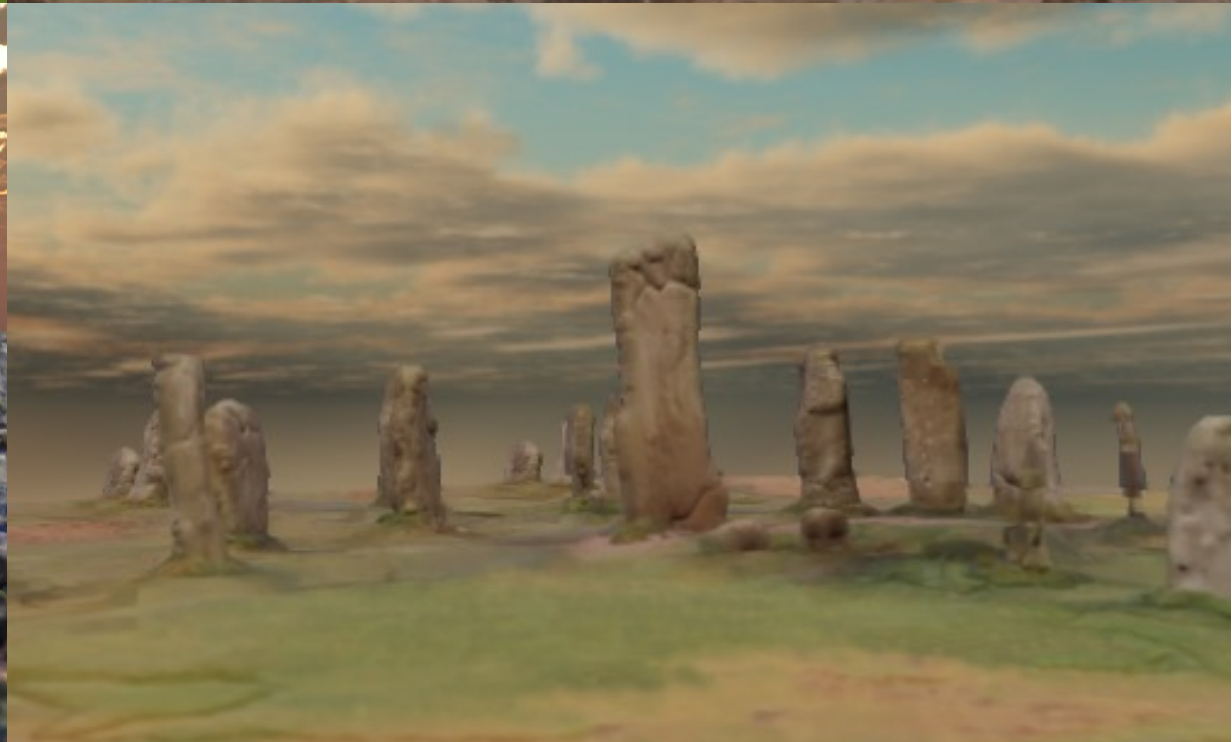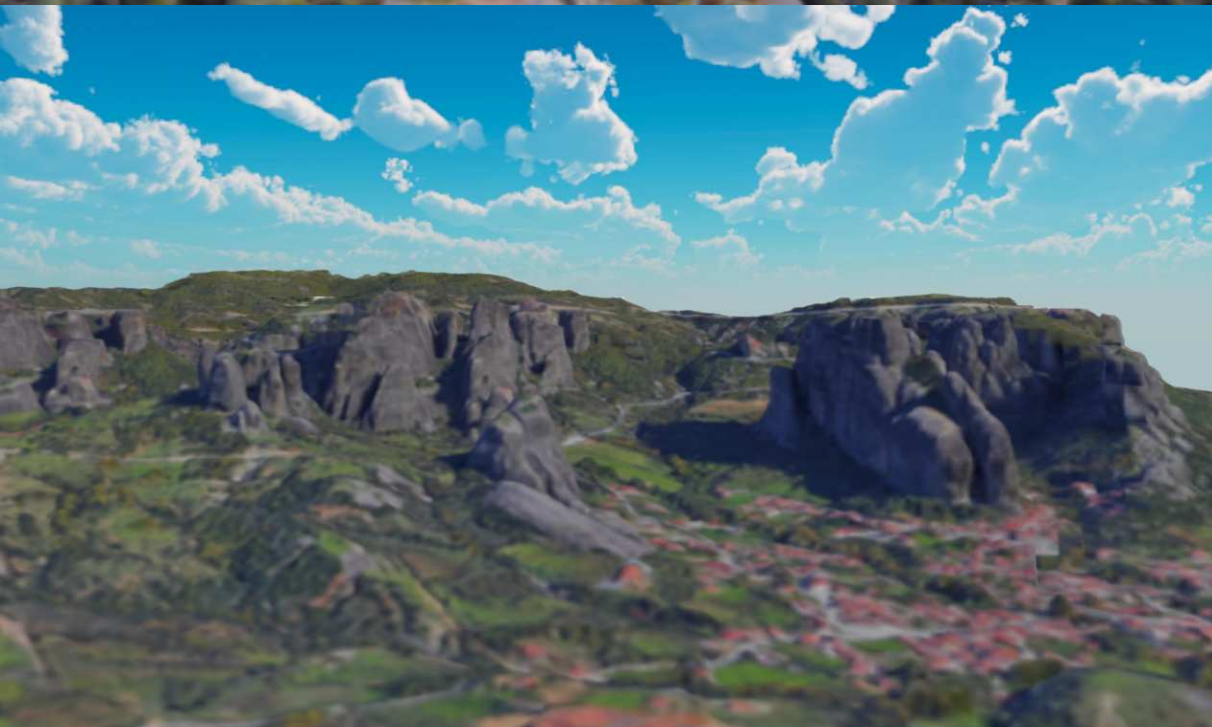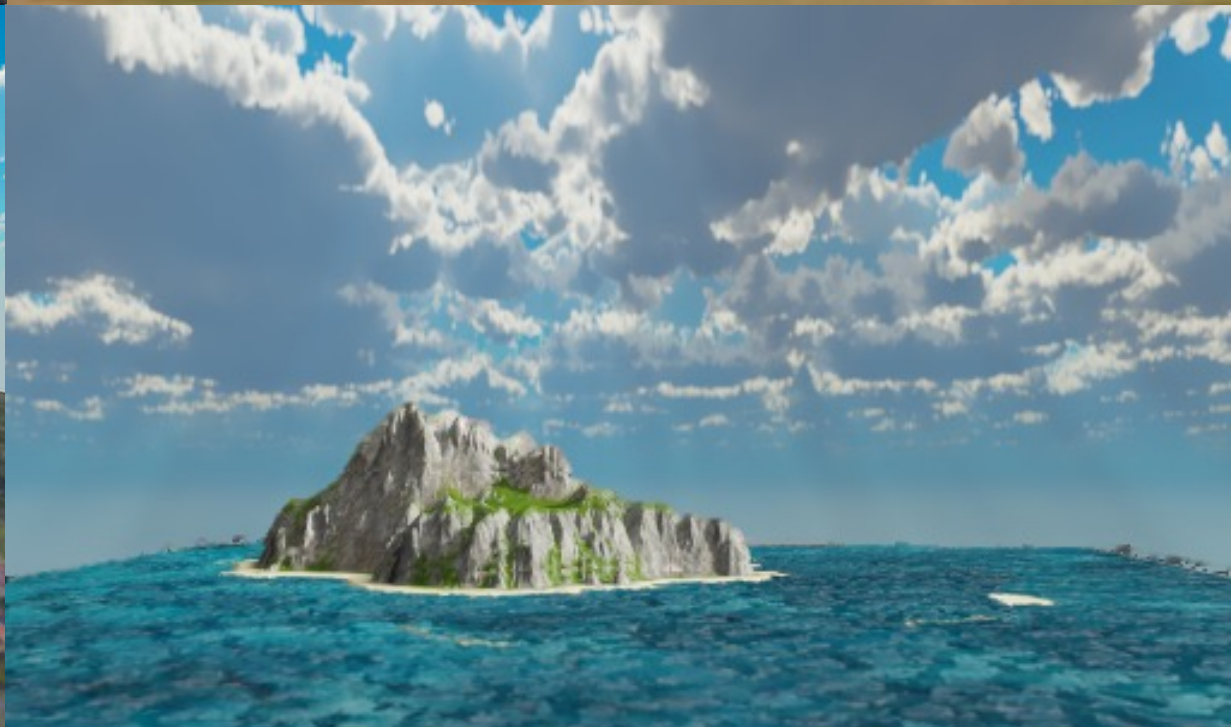

Supplement: Supplementary file 6 [file supplementary_teaser_long.pdf]
