# Supplementary material for: Patch-based 3D Natural Scene Generation from a Single Example
Source: arXiv:2304.12670 source file (2023-04-26)
Supplement: Supplementary file 7 [file supplementary_truncate_scale_effects.pdf]

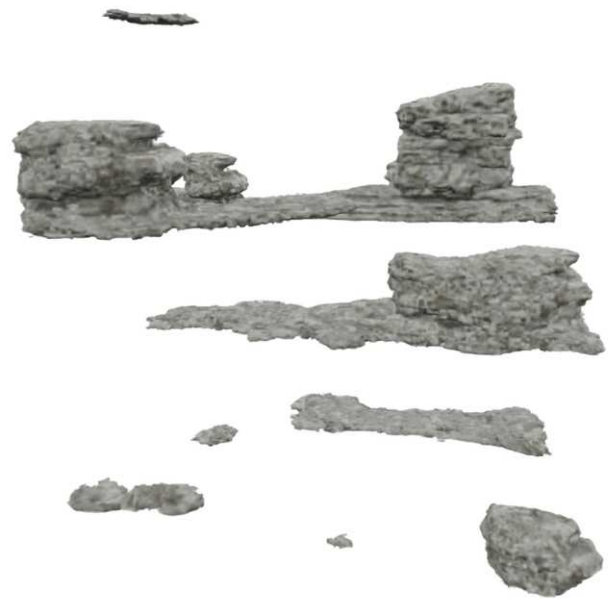

$$t = 1 \times w$$

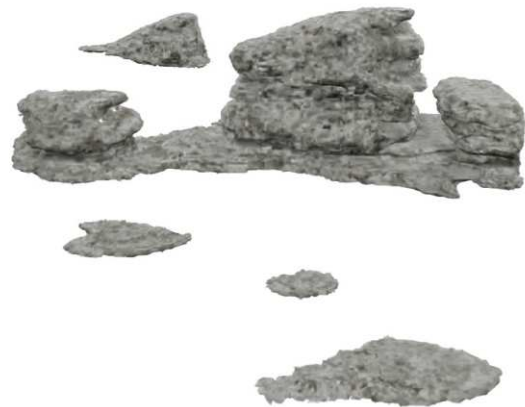

$$t = 2 \times w$$

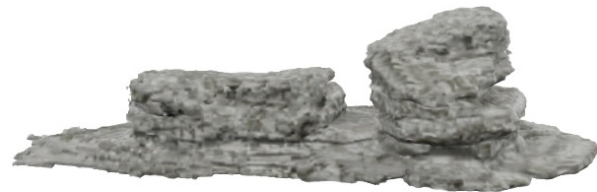

$$t = 4 \times w$$

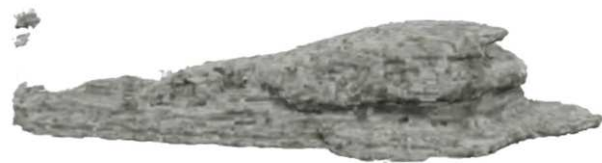

$$t = 8 \times w$$

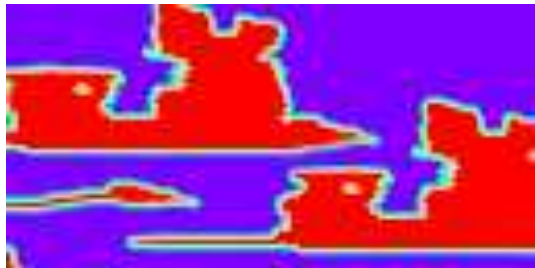

$$t = 1 \times w$$

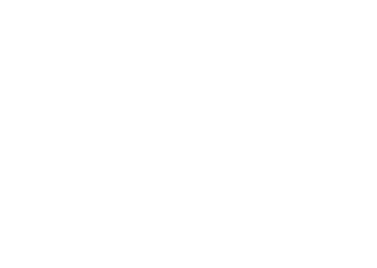

$$t = 2 \times w$$

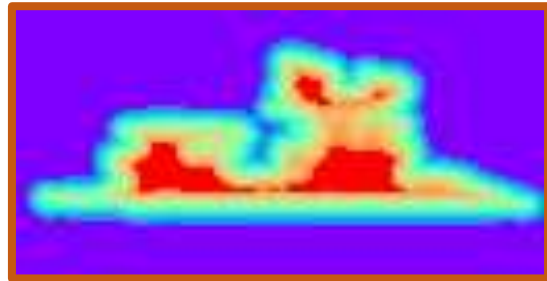

$$t = 4 \times w$$

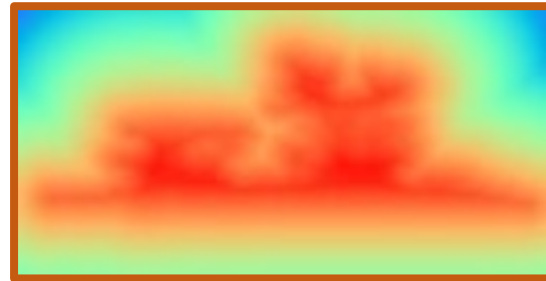

$$t = 8 \times w$$
